# Supplementary material for: High dimensional precision medicine from patient-derived xenografts
Source: arXiv:1912.06667 ancillary file (2019-12-13)
Supplement: Supplementary file 1 [file supplementary.pdf]

# Supplemental material for: High dimensional precision medicine from patient-derived xenografts

Naim U. Rashid[1,2], Jingxiang Chen[1], Michael T. Lawson[1], Daniel J. Luckett[1], Longshaokan Wang[7], Eric B. Laber[7], Yufeng Liu[1,3,4], Jen Jen Yeh[2,5,6], Donglin Zeng[1], and Michael R. Kosorok[1,4]

June 23, 2019

[1]Department of Biostatistics

[2]Lineberger Comprehensive Cancer Center

[3]Department of Statistics and Operations Research

[4]Department of Genetics

[5]Department of Surgery

[6]Department of Pharmacology

University of North Carolina at Chapel Hill

Chapel Hill, NC, USA

[7]Department of Statistics

North Carolina State University

Raleigh, NC, USA

# Contents

**1 Supplementary Figures** **2**

**2 Supplementary Tables** **15**

**3 Results for Best Average Response and $P_{opt}(\widehat{D}^*)$ Across Cancers (all methods)** **24**

**4 Results for Best Average Response and $P_{obs}(\widehat{D}^*)$** **30**

**5 Results for Log Time to Doubling and $P_{opt}(\widehat{D}^*)$** **37**

**6 Genomic platforms** **44**

6.1 RNA-seq . . . . . . . . . . . . . . . . . . . . . . . . . . . . . . . . . . . . . . . . 44

6.2 Copy Number data . . . . . . . . . . . . . . . . . . . . . . . . . . . . . . . . . . . 46

6.3 Mutation data . . . . . . . . . . . . . . . . . . . . . . . . . . . . . . . . . . . . . 47

**7 Supplementary Methods** **47**

7.1 Unsupervised Screening . . . . . . . . . . . . . . . . . . . . . . . . . . . . . . . . 47

7.2 Supervised Screening Based on Pairwise Treatment-Gene Interactions . . . . . . . . . . . . . 49

7.3 Dimension Reduction via Deep Learning . . . . . . . . . . . . . . . . . . . . . . . . 51

7.4 Adaptations of Off the Shelf Methods for ITR estimation . . . . . . . . . . . . . . . . 52

# 1 Supplementary Figures

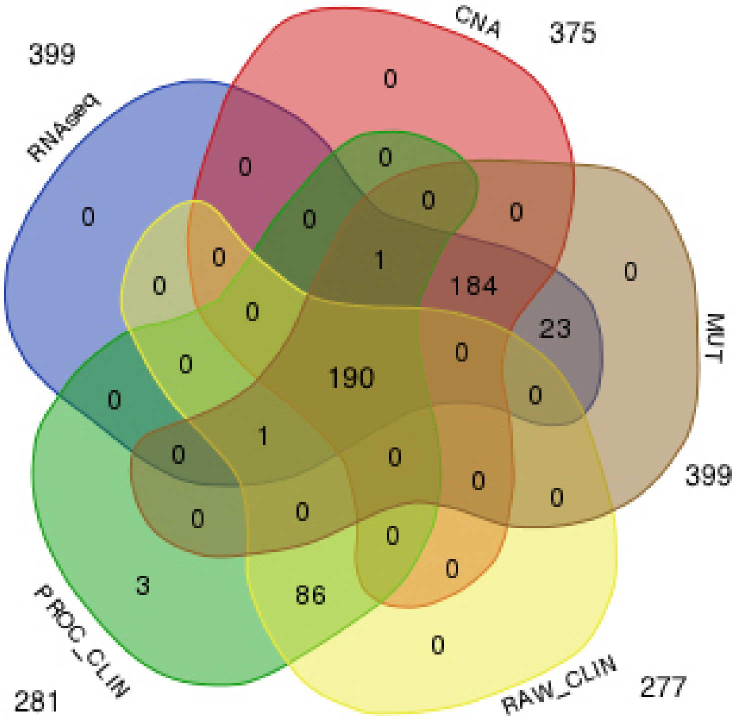


Figure 1: Genomic and response data availability corresponding to 488 PDX models. Out of a union set of 488 PDX models with data available to download, 190 had complete data over all possible data types. 184 PDX lines had complete genomic data but no clinical data.

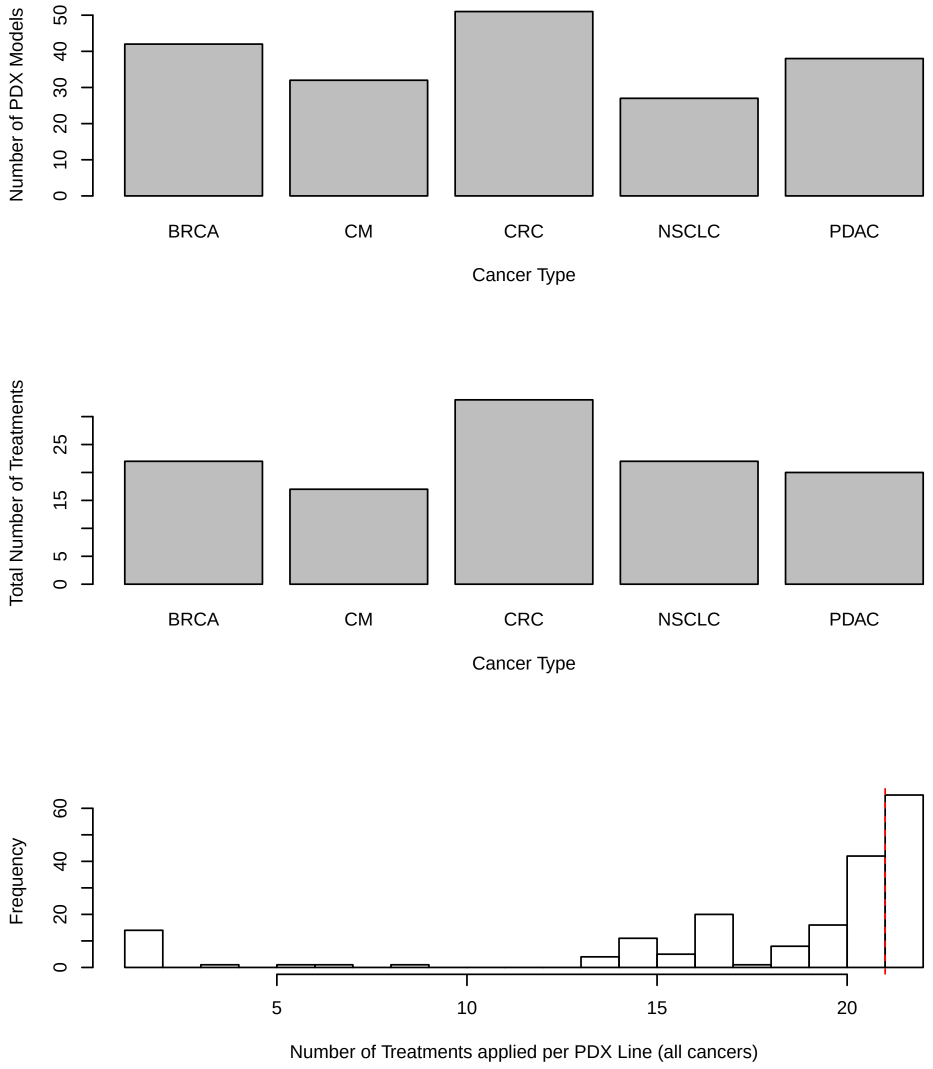


Figure 2: Total number of PDX lines per cancer, total number of treatments per cancer, and distribution of the number of treatments applied to each PDX line (median = 21 treatments, red dashed line). All values are those prior to treatment filtering.

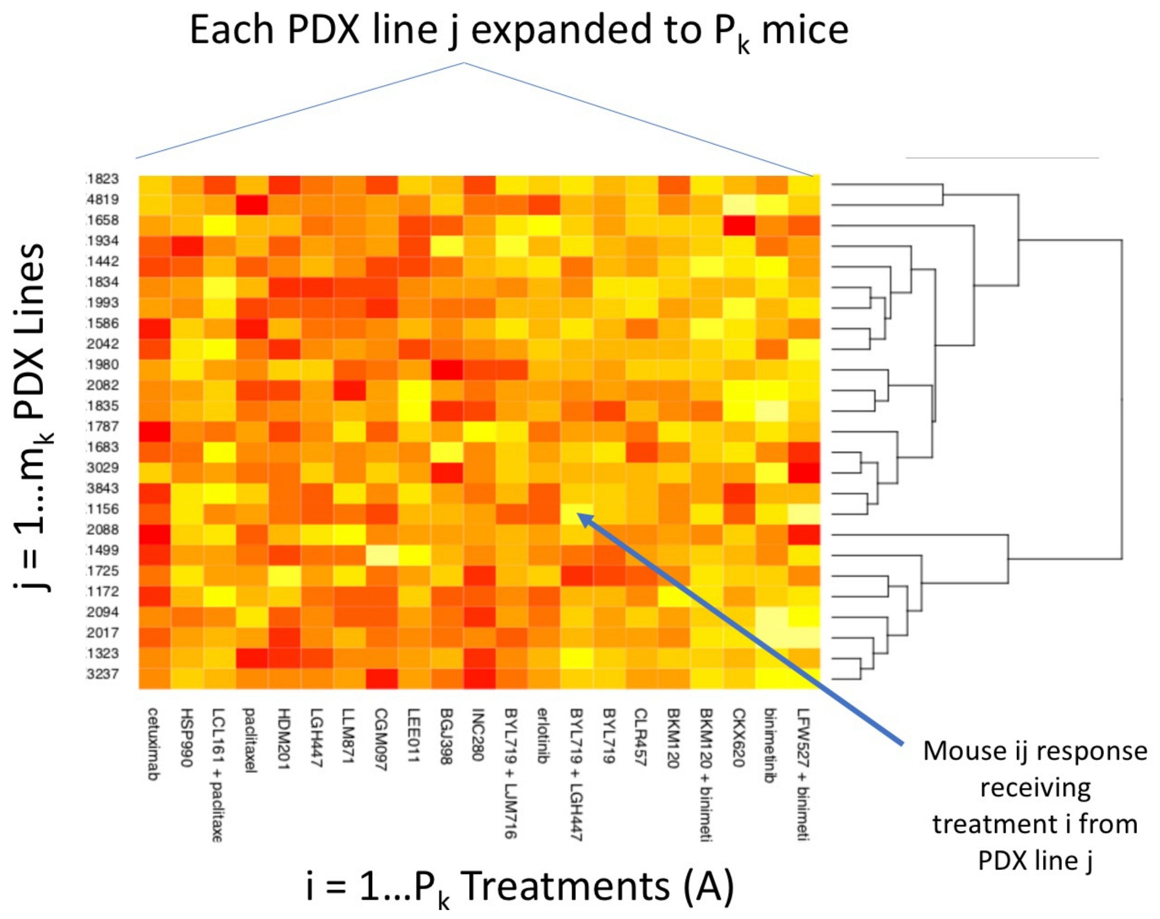


Figure 3: PDX Data Structure

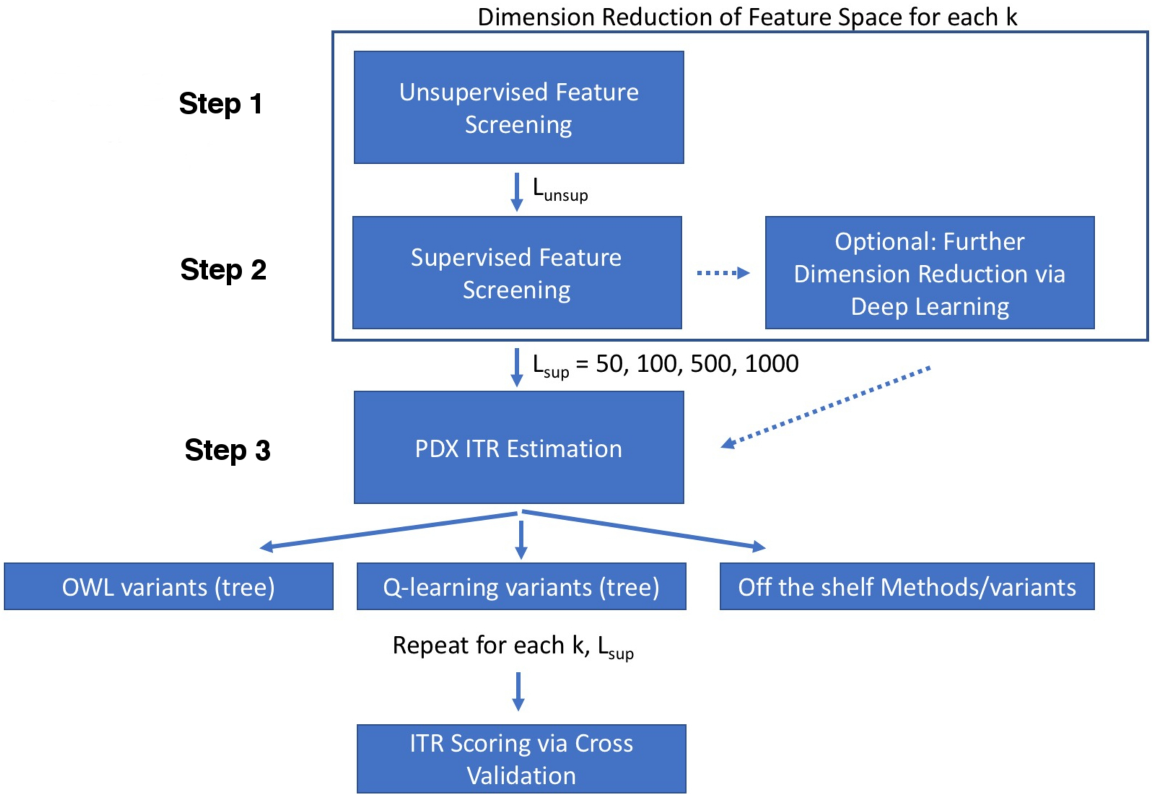


Figure 4: Overview of analytical pipeline

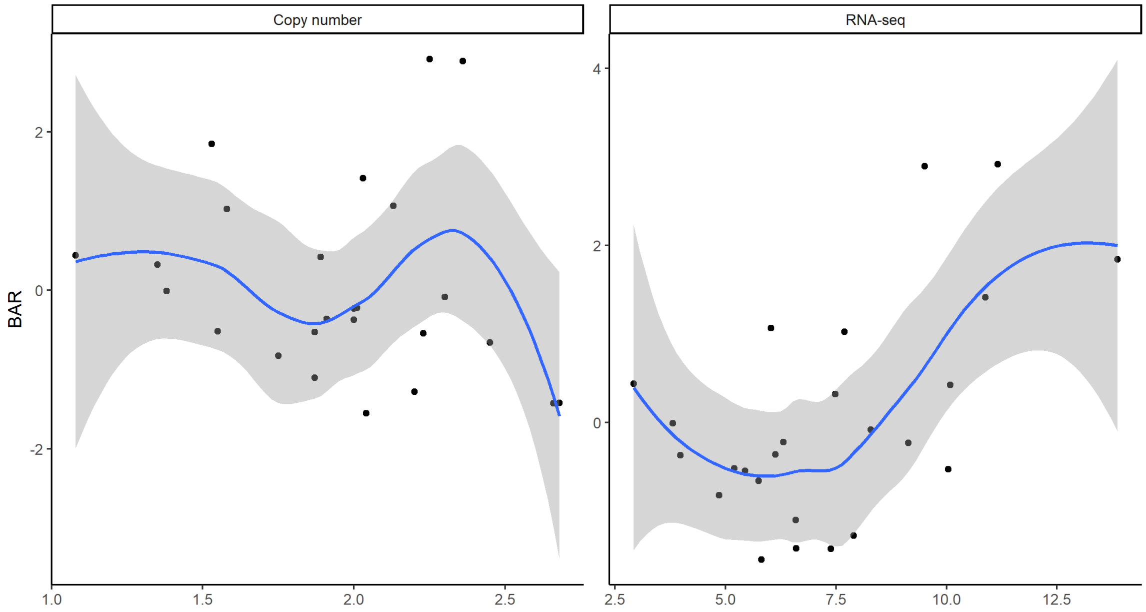


Figure 5: Example of non-linearity in the relationship between features and Binimetinib treatment response in NSCLC across PDX lines with respect to COX15 copy number (left) and COX15 RNA-seq gene expression (right).

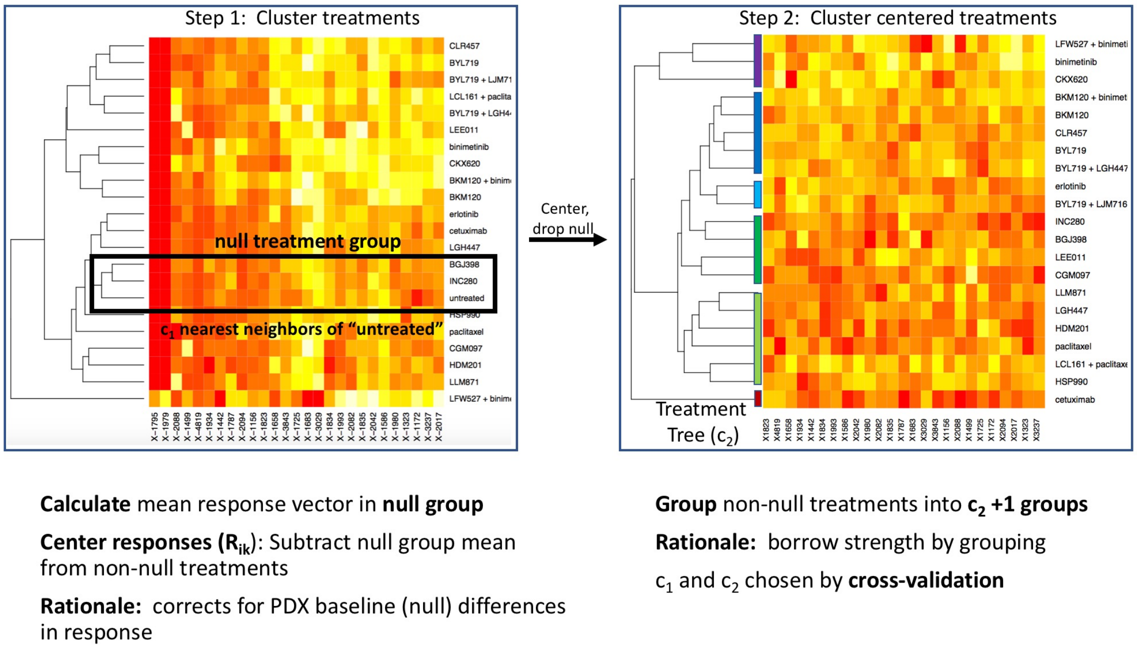


Figure 6: Overview of Treatment Tree Estimation

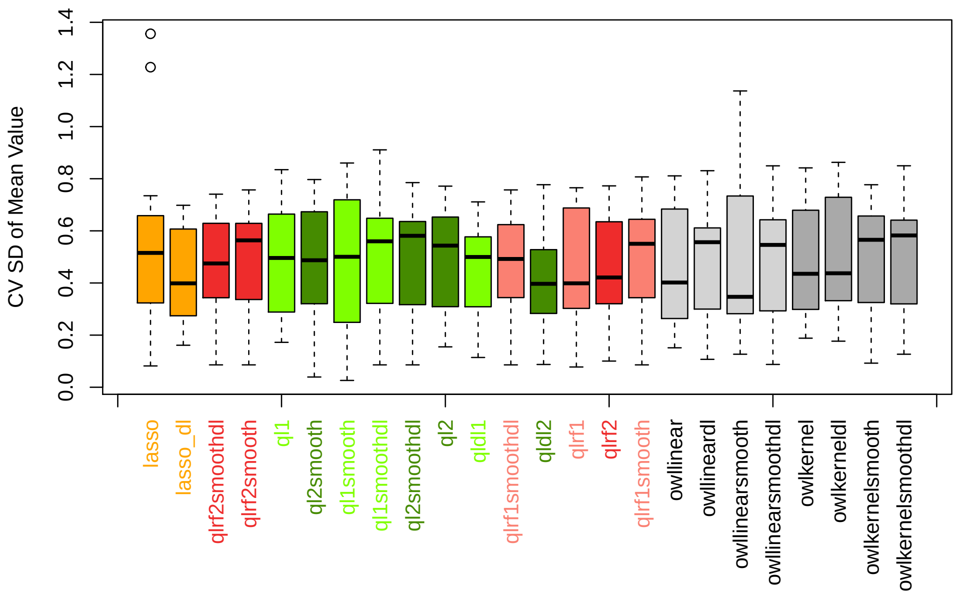


Figure 7: $\mathrm{sd}(\bar{V}(\widehat{D}^*))$ with respect to each method and their variants, pooled over cancer types and number of features utilized.

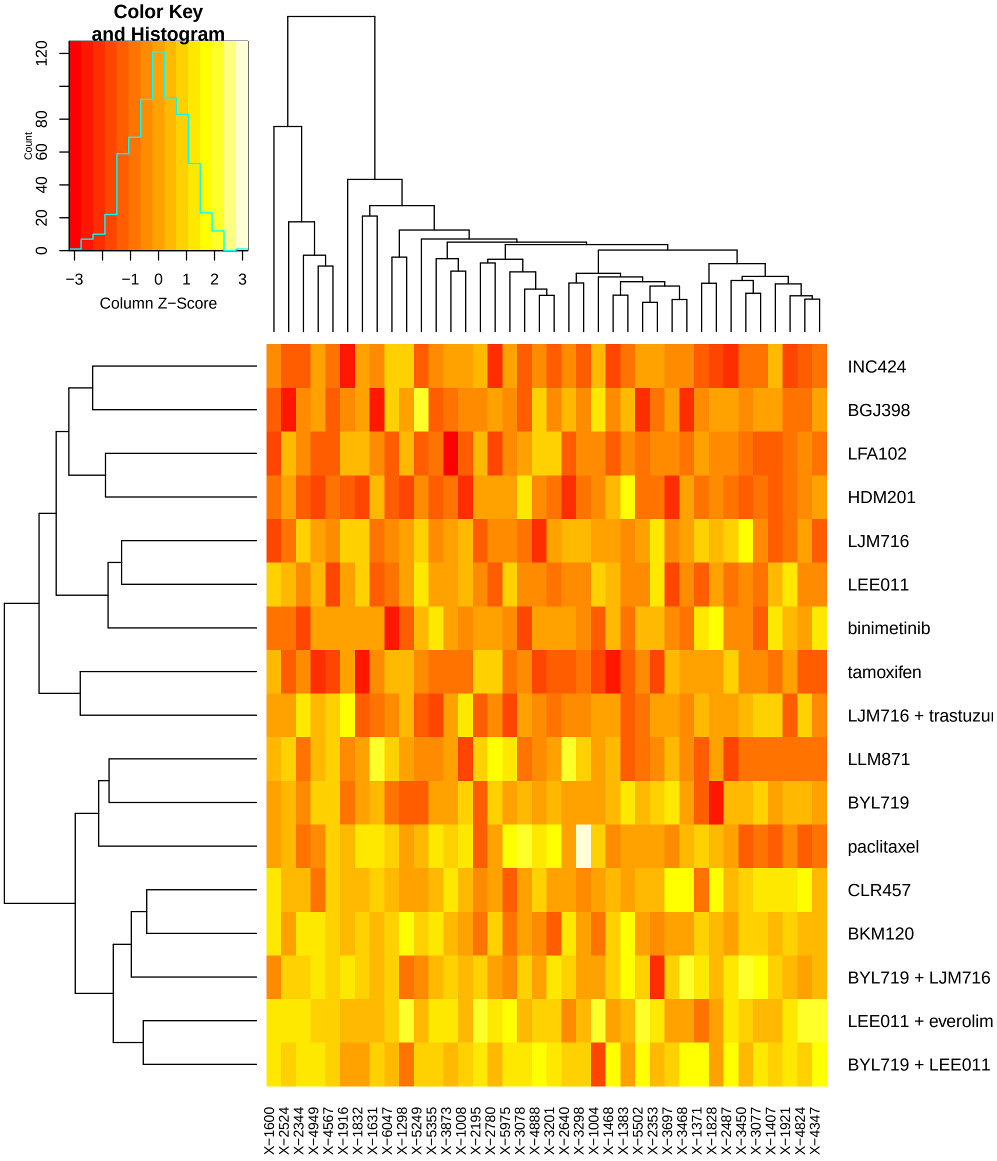


Figure 8: Clustered BRCA centered treatment response. Two treatments BYL719 + LJM716 and LEE011 + everolimus show very consistent performance across PDX lines relative to other treatments and outperforms all other methods.

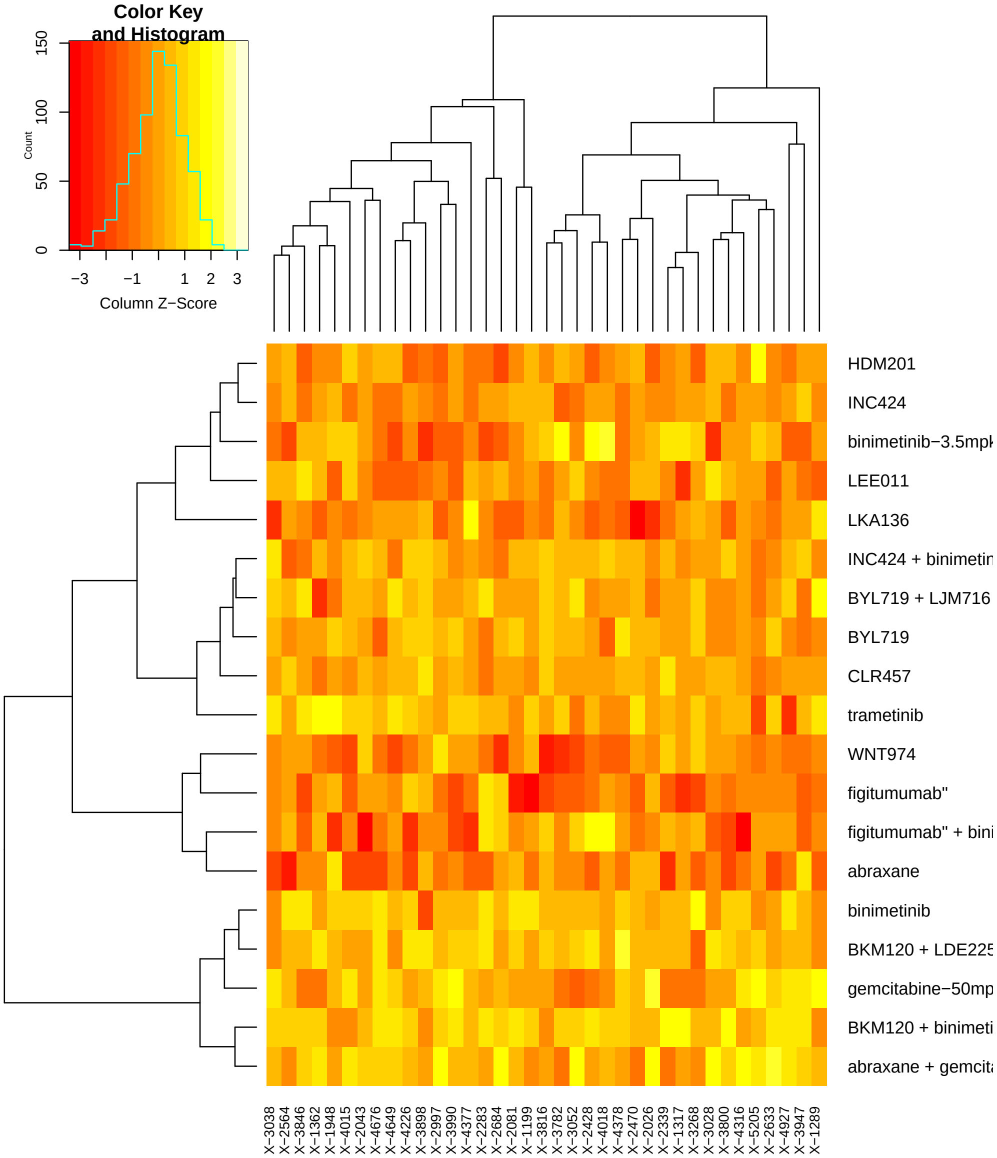


Figure 9: Significant heterogeneity in PDAC centered response observed across treatments, with no treatment consistently doing well across PDX lines

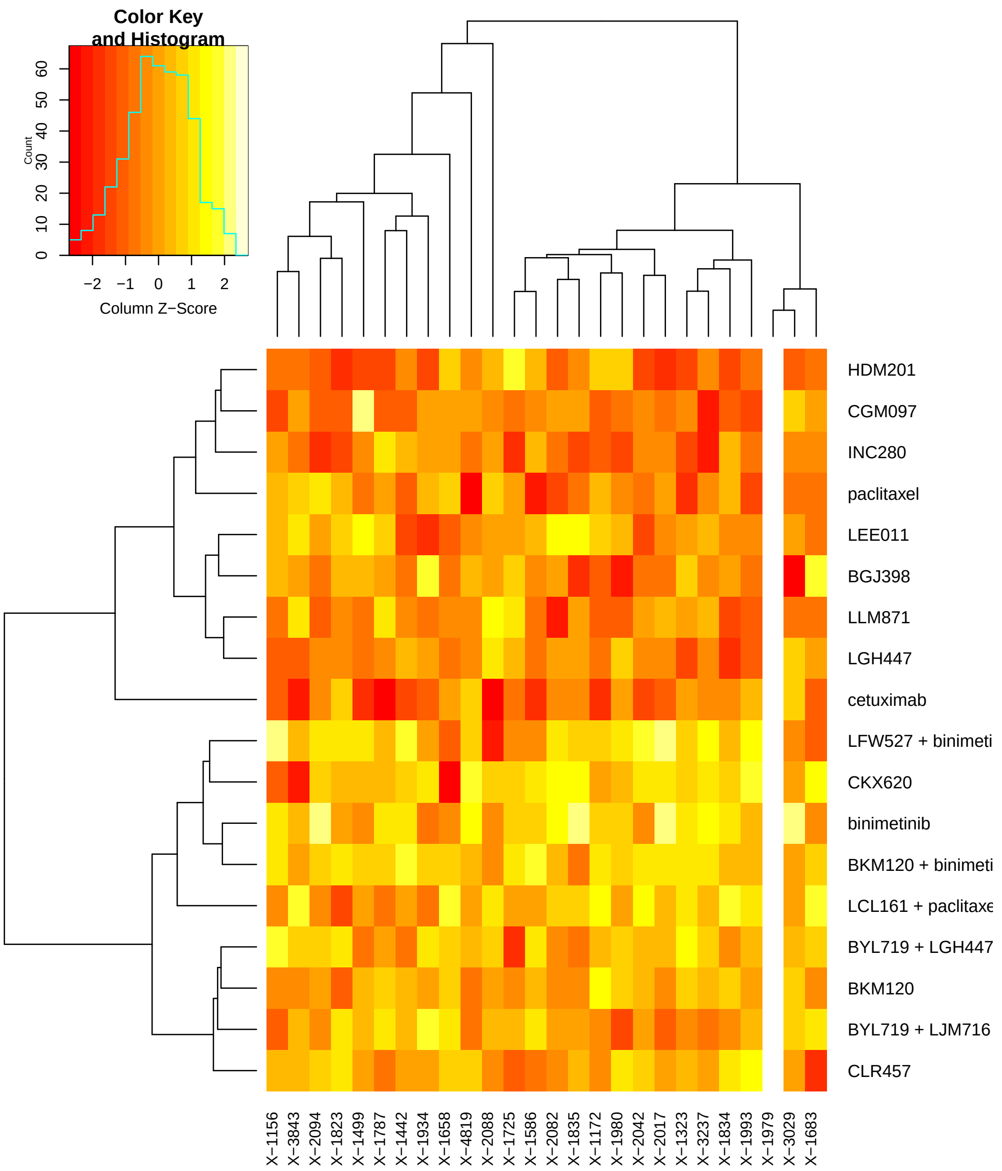


Figure 10: Significant heterogeneity in NSCLC centered response observed across treatments, with no treatment consistently doing well across PDX lines

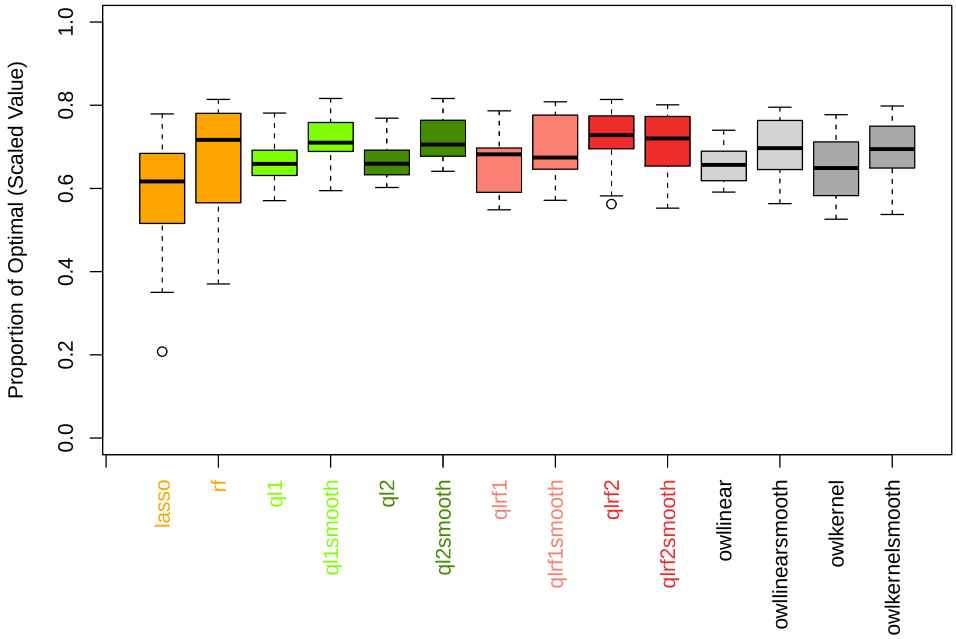


Figure 11: Overall performance with respect to each method and their variants (utilizing RNA-seq features only), pooled over cancer types and number of features utilized.

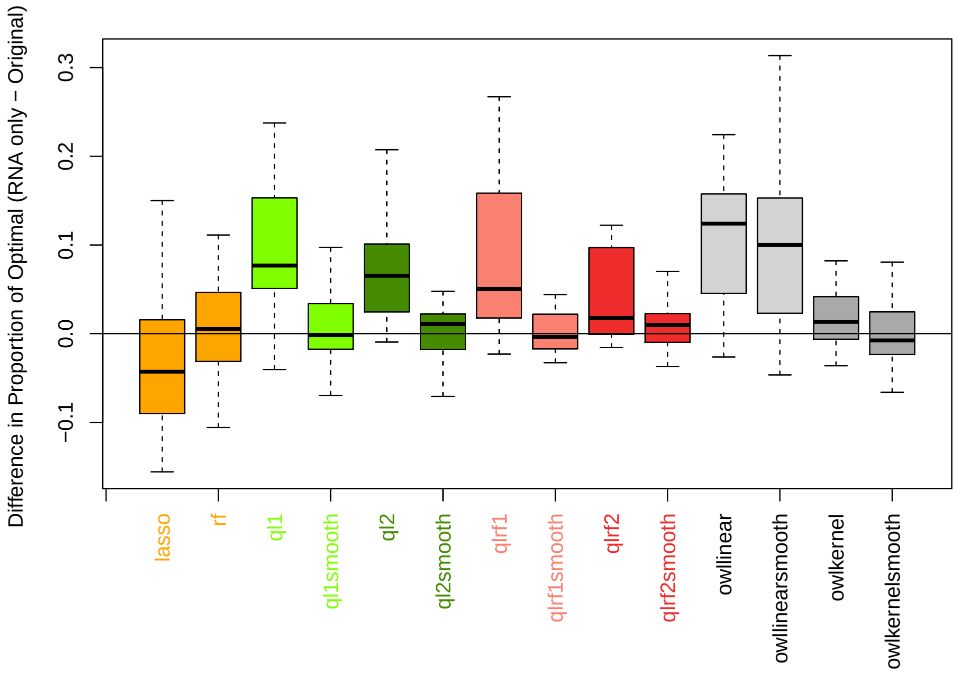


Figure 12: Overall difference in performance across methods and their variants, pooled over cancer types and number of features utilized. This difference is calculated for the optimal ITR from each method, method variance, and $L_{\text{LSUP}}$ value from the RNA-seq only analysis and the original analysis using features from all three genomics platforms.

# 2 Supplementary Tables

| Cancer | Max Trts | Max Trts/PDX | Filtered Trts /PDX | nPDXs | nPDXs After Filtering |
|---|---|---|---|---|---|
| BRCA | 22 | 22 | 22 | 42 | 38 |
| CRC | 34 | 22 | 22 | 51 | 43 |
| NSCLC | 22 | 22 | 22 | 27 | 25 |
| PDAC | 21 | 21 | 21 | 38 | 38 |
| CM | 17 | 17 | 17 | 32 | 32 |

Table 1: For each cancer we detail the maximum number of treatments applied to PDX models, the maximum number of PDX models per treatment, the number of treatments remaining after filtering, total number of PDX lines, and the number of PDX Lines with greater than one mouse receiving treatment

| | BRCA | CM | CRC | NSCLC | PDAC |
|---|---|---|---|---|---|
| $L_{\text{UNSUP}}$ | 21947 | 22014 | 22014 | 22011 | 22012 |
| $p_{\text{UNSUP}}$ | 32739 | 32753 | 32769 | 32812 | 32665 |
| $p_{\text{UNSUP,RNA}}$ | 13577 | 13577 | 13577 | 13577 | 13577 |
| $p_{\text{UNSUP,CN}}$ | 18868 | 18868 | 18868 | 18868 | 18868 |
| $p_{\text{UNSUP,MUT}}$ | 294 | 308 | 324 | 367 | 220 |
| $p_{L_{\text{SUP}}}$ 50 | 95 | 91 | 94 | 92 | 111 |
| $p_{L_{\text{SUP}}}$ 100 | 187 | 157 | 167 | 158 | 166 |
| $p_{L_{\text{SUP}}}$ 500 | 835 | 691 | 658 | 683 | 751 |
| $p_{L_{\text{SUP}}}$ 1000 | 1638 | 1346 | 1279 | 1398 | 1547 |

Table 2: For each cancer we detail the number of genes $L_{\text{UNSUP}}$ and the number of corresponding features $p_{\text{UNSUP}}$ remaining after unsupervised screening, the latter broken down by genomic platform. We also detail the total number of features remaining after supervised screening $p_{L_{\text{SUP}}}$, which is indexed by the value of $L_{\text{SUP}}$, which is the number of genes remaining after supervised screening with at least one feature. We note that $L_{\text{UNSUP}} \neq p_{L_{\text{SUP}}}$ as each gene may have up to 3 possible features (one from each genomic platform) following the unsupervised screening. More details on this screening are given in Supplementary Material Section 7.

| | 50 | 100 | 500 | 1000 |
|---|---|---|---|---|
| BRCA | 0.065126 | 0.000000 | 0.000000 | 0.000000 |
| CM | 0.077983 | 0.000002 | 0.000002 | 0.000001 |
| CRC | 0.232212 | 0.107321 | 0.000000 | 0.074550 |
| NSCLC | 0.015293 | 0.019432 | 0.020588 | 0.021317 |
| PDAC | 0.134007 | 0.000000 | 0.000000 | 0.000000 |

Table 3: Reconstruction Error of Deep Learning Autoencoders. Within each cancer, we obtain four screened feature sets of increasing dimension, indexed by $LSUP$, where $LSUP = 50, 100, 500, 1000$. We apply Deep Learning Autoencoders to reduce the dimension of each screened set within each cancer (final dimension chosen by cross validation given in Supplementary Table 5). Here we list the calculated reconstruction error for each set as a measure of accuracy, where reconstruction error is the squared distance between the original data and its "estimate" after dimension reduction

| | 50 | 100 | 500 | 1000 |
|---|---|---|---|---|
| BRCA | 0.128740 | 0.209583 | 0.000000 | 0.000000 |
| CM | 0.349320 | 0.249223 | 0.000000 | 0.000000 |
| CRC | 0.468226 | 0.391763 | 0.137462 | 0.000000 |
| NSCLC | 0.324879 | 0.454082 | 0.017193 | 0.018317 |
| PDAC | 0.430976 | 0.355374 | 0.449184 | 0.098939 |

Table 4: Reconstruction error of PCA. Within each cancer, we obtain four screened feature sets of increasing dimension, indexed by $LSUP$, where $LSUP = 50, 100, 500, 1000$. We apply PCA to reduce the dimension of each screened set within each cancer. Here we list the calculated reconstruction error for each set as a measure of accuracy, where reconstruction error is the squared distance between the original data and its "estimate" after dimension reduction. We find that the reconstruction error for each set is in general similar or larger than that observed by deep learning. These results motivate our use of deep learning autoencoders for dimension reduction in our evaluations.

| | 50 | 100 | 500 | 1000 |
|---|---|---|---|---|
| BRCA | 10 | 10 | 9 | 17 |
| CM | 5 | 8 | 7 | 14 |
| CRC | 19 | 9 | 33 | 13 |
| NSCLC | 18 | 32 | 137 | 140 |
| PDAC | 12 | 9 | 8 | 16 |

Table 5: Selected dimension of each predictor set (indexed by LSUP) within each cancer following dimesion reduction by Deep Learning Autoencoders. Within each cancer, we obtain the original four screened feature sets of increasing dimension and then apply deep learning autoencoders to reduce the dimension from $p_{L_{SUP}}$ (see Supplementary Table 2) to the values provided in this table. The final dimension of each predictor set is chosen by cross validation.

| Cancer | Method | Lsup | c_1 | c_2+1 | Most Rec | PDX Rec | 2nd Most Rec | PDX Rec (2nd) |
|---|---|---|---|---|---|---|---|---|
| BRCA | owllinearsmoothdl | 50 | 3 | 17 | LEE011 + everolimus | 17/38 | BYL719 + LEE011 | 16/38 |
| CM | owllineardl | 100 | 2 | 9 | LEE011 + encorafenib | 20/32 | BKM120 + encorafenib | 12/32 |
| CRC | ql1smooth | 100 | 3 | 17 | BYL719 + binimetinib | 43/43 | | NA/43 |
| NSCLC | owlkernelsmooth | 100 | 3 | 14 | binimetinib | 24/50 | BKM120 + binimetinib | 24/50 |
| PDAC | ql1smooth | 100 | 1 | 18 | abraxane + gemcitabine | 18/37 | BKM120 + binimetinib | 18/37 |

Table 6: For the optimal ITR from each cancer, we list the method's corresponding $c_1$ for its estimated treatment tree (number of treatments grouped with "untreated" to form the null treatments group), $c_2 + 1$ (the number of non-null treatments after recentering), the most recommended treatment group for that method (Most Rec), the number of PDX lines for that cancer that the treatment group was recommended for (PDX Rec), and the second place method (2nd Most Rec, PDX Rec 2nd).

| Cancer | Treatment Group | Frequency |
|---|---|---|
| BRCA | LEE011 + everolimus | 17 |
| BRCA | BYL719 + LEE011 | 16 |
| BRCA | BYL719 + LJM716 | 4 |
| BRCA | paclitaxel | 1 |
| CM | LEE011 + encorafenib | 20 |
| CM | BKM120 + encorafenib | 12 |
| CRC | BYL719 + binimetinib | 43 |
| NSCLC | binimetinib | 24 |
| NSCLC | BKM120 + binimetinib | 24 |
| NSCLC | LFW527 + binimetinib | 2 |
| PDAC | abraxane + gemcitabine | 18 |
| PDAC | BKM120 + binimetinib | 18 |
| PDAC | gemcitabine-50mpk | 1 |

Table 7: For the optimal ITR from each cancer, we list each method's set of recommended treatments. Treatments that were never recommended by the optimal ITR are omitted.

| Cancer | Treatment | Average Response | Standard Error |
|---|---|---|---|
| BRCA | LEE011 + everolimus | 1.45 | 0.19 |
| BRCA | BYL719 + LEE011 | 1.38 | 0.18 |
| BRCA | BYL719 + LJM716 | 1.26 | 0.16 |
| BRCA | BKM120 | 1.19 | 0.17 |
| BRCA | CLR457 | 1.14 | 0.16 |
| BRCA | paclitaxel | 1.1 | 0.17 |
| BRCA | LLM871 | 0.87 | 0.2 |
| BRCA | BYL719 | 0.85 | 0.18 |
| BRCA | LJM716 | 0.8 | 0.12 |
| BRCA | LEE011 | 0.78 | 0.17 |
| BRCA | LJM716 + trastuzumab | 0.78 | 0.19 |
| BRCA | binimetinib | 0.71 | 0.14 |
| BRCA | BGJ398 | 0.57 | 0.15 |
| BRCA | LFA102 | 0.43 | 0.16 |
| BRCA | tamoxifen | 0.43 | 0.18 |
| BRCA | INC424 | 0.42 | 0.18 |
| BRCA | CGM097 | 0.41 | 0.15 |
| BRCA | HDM201 | 0.38 | 0.17 |
| BRCA | LKA136 | 0.27 | 0.12 |
| BRCA | trastuzumab | 0.19 | 0.17 |
| BRCA | untreated | 0 | 0 |
| CM | LEE011 + encorafenib | 2.26 | 0.3 |
| CM | BKM120 + encorafenib | 2.11 | 0.36 |
| CM | encorafenib + binimetinib | 2 | 0.3 |
| CM | binimetinib | 1.77 | 0.24 |

| | | | |
|---|---|---|---|
| CM | dacarbazine | 1.55 | 0.34 |
| CM | BKM120 | 1.43 | 0.26 |
| CM | LEE011 | 1.42 | 0.26 |
| CM | TAS266 | 1.33 | 0.3 |
| CM | encorafenib | 1.11 | 0.28 |
| CM | CGM097 | 1.08 | 0.27 |
| CM | LDE225 | 1.01 | 0.27 |
| CM | LGW813 | 1.01 | 0.27 |
| CM | LDK378 | 0.9 | 0.22 |
| CM | WNT974 | 0.59 | 0.31 |
| CM | untreated | 0 | 0 |
| CRC | BYL719 + binimetinib | 0.99 | 0.15 |
| CRC | BYL719 + LJM716 | 0.9 | 0.16 |
| CRC | CLR457 | 0.82 | 0.14 |
| CRC | CKX620 | 0.77 | 0.16 |
| CRC | BYL719 + cetuximab | 0.71 | 0.14 |
| CRC | binimetinib | 0.64 | 0.18 |
| CRC | BKM120 | 0.61 | 0.17 |
| CRC | BYL719 + cetuximab + encorafenib | 0.61 | 0.16 |
| CRC | BYL719 | 0.59 | 0.17 |
| CRC | 5FU | 0.58 | 0.13 |
| CRC | LEE011 | 0.57 | 0.15 |
| CRC | cetuximab | 0.42 | 0.18 |
| CRC | BYL719 + encorafenib | 0.39 | 0.16 |
| CRC | cetuximab + encorafenib | 0.29 | 0.19 |
| CRC | BKM120 + LJC049 | 0.25 | 0.21 |
| CRC | HDM201 | 0.12 | 0.16 |

| | | | |
|---|---|---|---|
| CRC | CGM097 | 0.04 | 0.18 |
| CRC | LKA136 | 0.03 | 0.15 |
| CRC | untreated | 0 | 0 |
| CRC | encorafenib | -0.11 | 0.16 |
| CRC | LJC049 | -0.15 | 0.21 |
| NSCLC | binimetinib | 1.34 | 0.27 |
| NSCLC | BKM120 + binimetinib | 1.28 | 0.2 |
| NSCLC | CKX620 | 1.22 | 0.33 |
| NSCLC | LCL161 + paclitaxel | 1.2 | 0.3 |
| NSCLC | LFW527 + binimetinib | 1.12 | 0.31 |
| NSCLC | BYL719 + LGH447 | 1.08 | 0.24 |
| NSCLC | BKM120 | 0.9 | 0.25 |
| NSCLC | CLR457 | 0.9 | 0.16 |
| NSCLC | BYL719 + LJM716 | 0.88 | 0.24 |
| NSCLC | BYL719 | 0.86 | 0.19 |
| NSCLC | HSP990 | 0.84 | 0.28 |
| NSCLC | erlotinib | 0.74 | 0.22 |
| NSCLC | LEE011 | 0.7 | 0.32 |
| NSCLC | BGJ398 | 0.56 | 0.25 |
| NSCLC | LLM871 | 0.54 | 0.33 |
| NSCLC | LGH447 | 0.5 | 0.29 |
| NSCLC | CGM097 | 0.31 | 0.28 |
| NSCLC | paclitaxel | 0.3 | 0.31 |
| NSCLC | INC280 | 0.26 | 0.24 |
| NSCLC | HDM201 | 0.17 | 0.28 |
| NSCLC | untreated | 0 | 0 |
| NSCLC | cetuximab | -0.1 | 0.24 |

| | | | |
|---|---|---|---|
| PDAC | BKM120 + binimetinib | 0.95 | 0.15 |
| PDAC | abraxane + gemcitabine | 0.8 | 0.17 |
| PDAC | BKM120 + LDE225 | 0.79 | 0.13 |
| PDAC | binimetinib | 0.76 | 0.13 |
| PDAC | gemcitabine-50mpk | 0.63 | 0.18 |
| PDAC | BYL719 + LJM716 | 0.55 | 0.13 |
| PDAC | INC424 + binimetinib | 0.55 | 0.14 |
| PDAC | trametinib | 0.55 | 0.12 |
| PDAC | BYL719 | 0.39 | 0.13 |
| PDAC | CLR457 | 0.32 | 0.11 |
| PDAC | BKM120 | 0.24 | 0.12 |
| PDAC | binimetinib-3.5mpk | 0.13 | 0.17 |
| PDAC | INC424 | 0.09 | 0.14 |
| PDAC | HDM201 | 0.09 | 0.16 |
| PDAC | LEE011 | 0.08 | 0.14 |
| PDAC | LKA136 | 0.01 | 0.12 |
| PDAC | untreated | 0 | 0 |
| PDAC | figitumumab" + binimetinib | -0.11 | 0.19 |
| PDAC | WNT974 | -0.11 | 0.13 |
| PDAC | figitumumab" | -0.2 | 0.18 |
| PDAC | abraxane | -0.26 | 0.16 |

Table 8: Average centered treatment effect for each cancer and treatment with estimated standard errors.

# 3 Results for Best Average Response and $P_{opt}(\widehat{D}^*)$ Across Cancers (all methods)

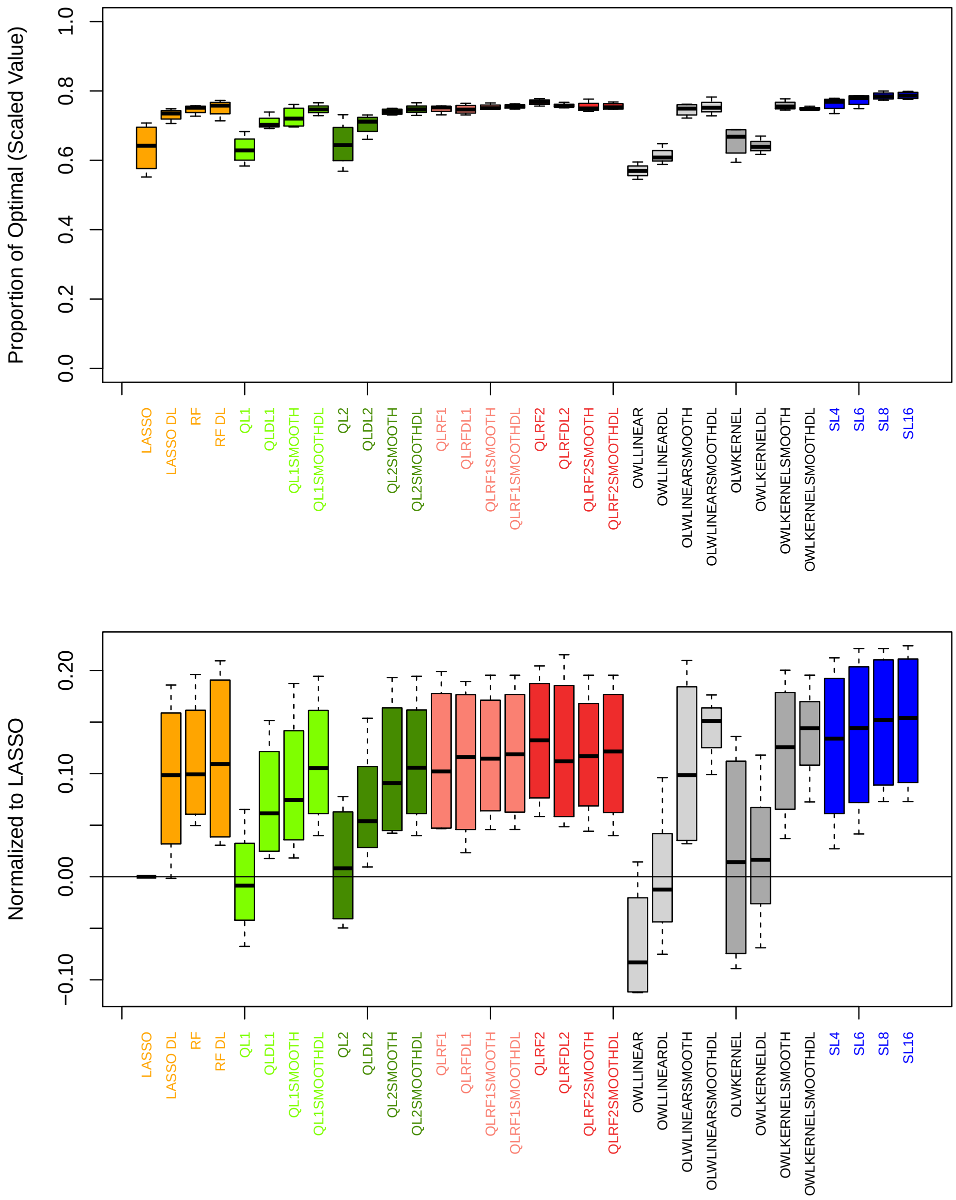


Figure 13: Overall performance with respect to each method and their variants in BRCA, pooled over cancer types and number of features utilized (top). $P_{opt}(\widehat{D}^*)$ for each method is normalized to the LASSO in each condition to highlight the relative performance of each approach (bottom). This relative measure was constructed by subtracting the $P_{opt}(\widehat{D}^*)$ pertaining to the LASSO from that of the other methods within each combination of cancer type and $L_{\text{SUP}}$ value.

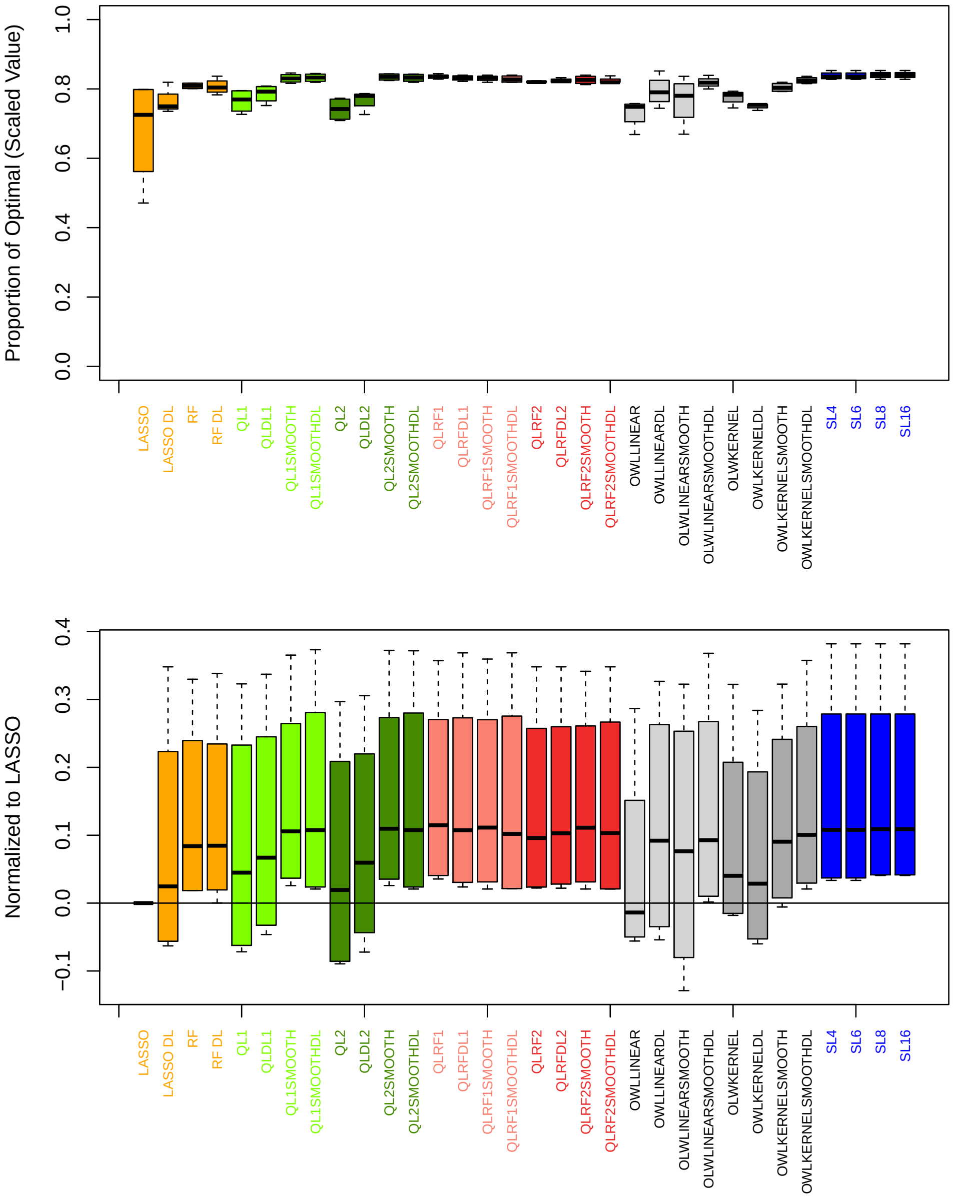


Figure 14: Overall performance with respect to each method and their variants in CM, pooled over cancer types and number of features utilized (top). $P_{opt}(\widehat{D}^*)$ for each method is normalized to the LASSO in each condition to highlight the relative performance of each approach (bottom). This relative measure was constructed by subtracting the $P_{opt}(\widehat{D}^*)$ pertaining to the LASSO from that of the other methods within each combination of cancer type and $L_{\text{SUP}}$ value.

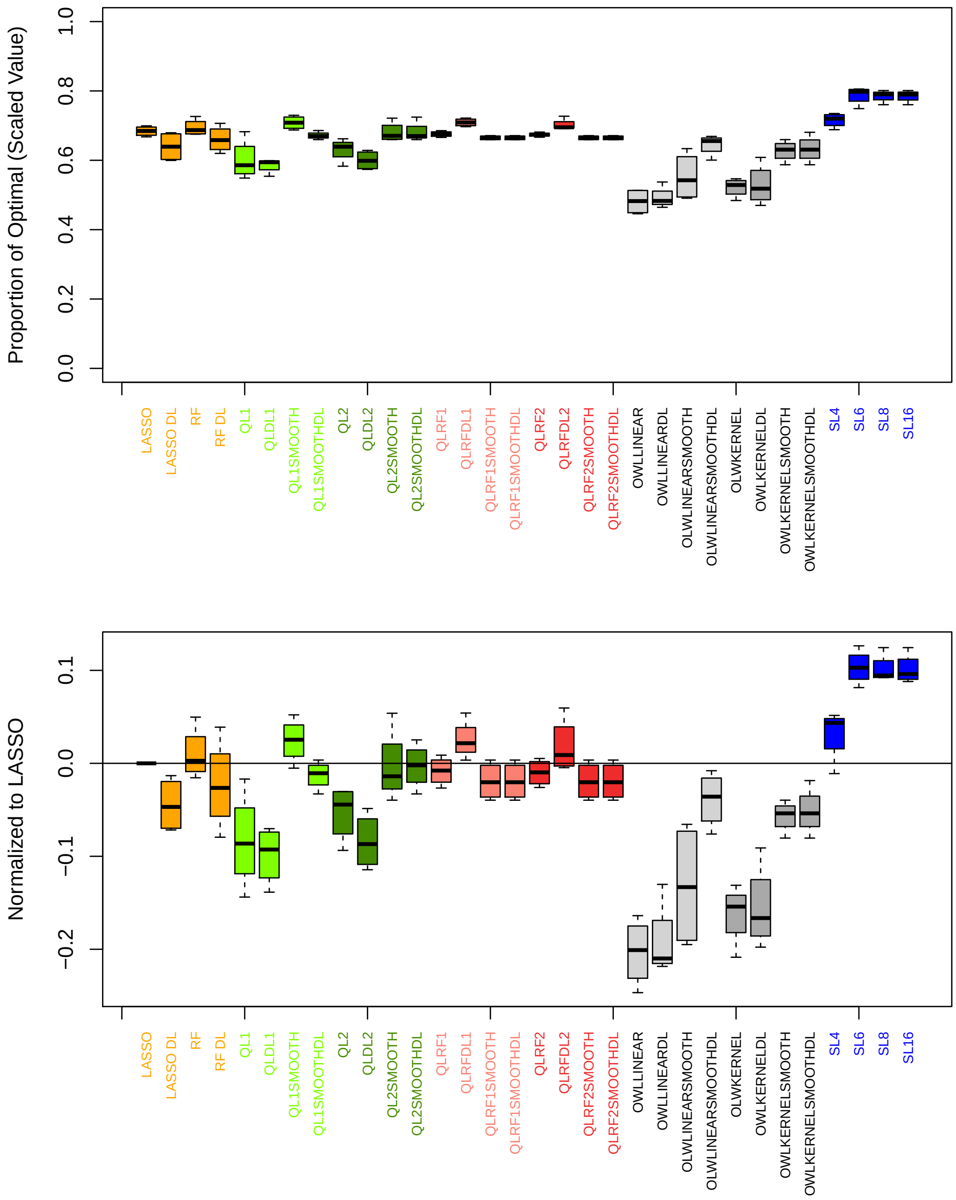


Figure 15: Overall performance with respect to each method and their variants in CRC, pooled over cancer types and number of features utilized (top). $P_{opt}(\widehat{D}^*)$ for each method is normalized to the LASSO in each condition to highlight the relative performance of each approach (bottom). This relative measure was constructed by subtracting the $P_{opt}(\widehat{D}^*)$ pertaining to the LASSO from that of the other methods within each combination of cancer type and $L_{\text{SUP}}$ value.

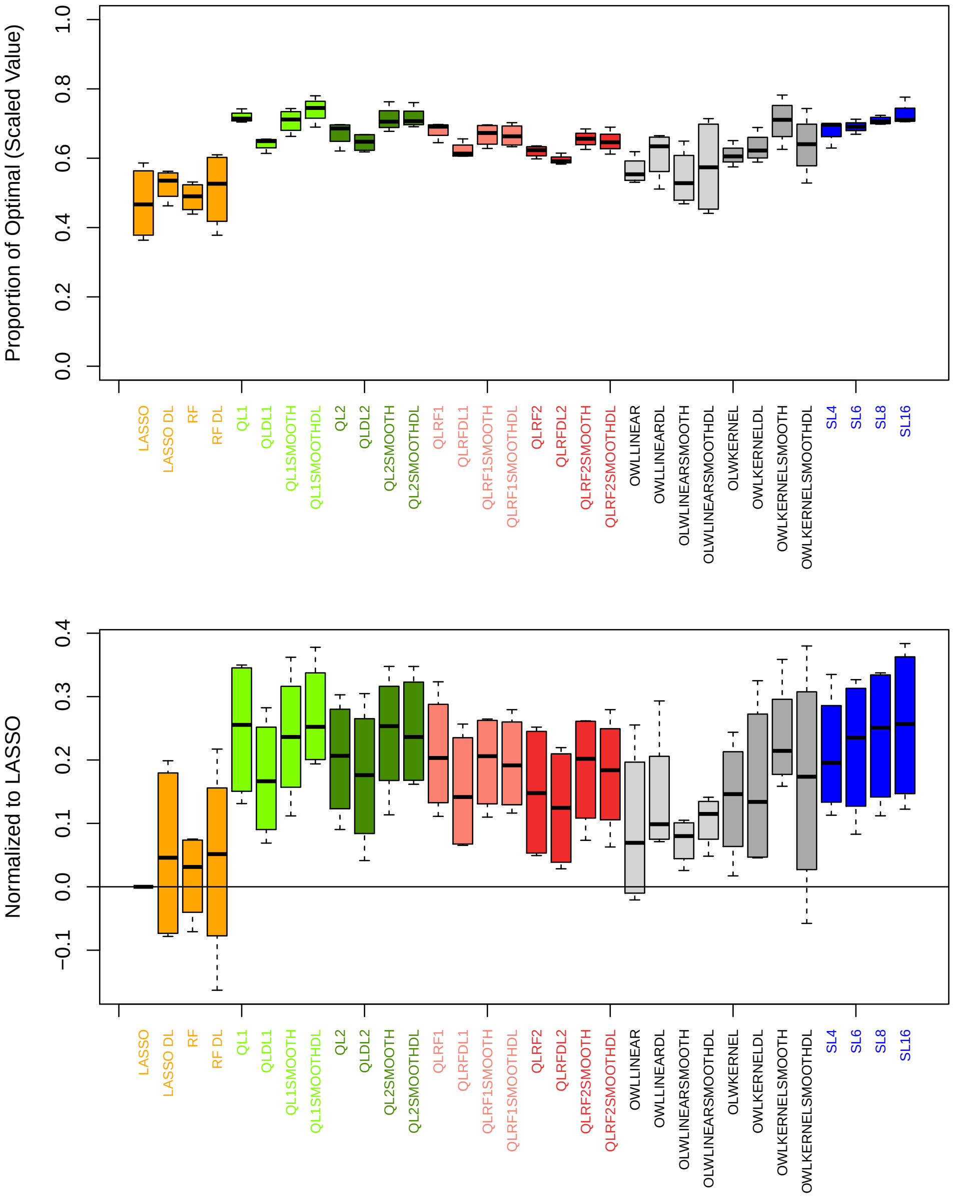


Figure 16: Overall performance with respect to each method and their variants in NSCLC, pooled over cancer types and number of features utilized (top). $P_{opt}(\widehat{D}^*)$ for each method is normalized to the LASSO in each condition to highlight the relative performance of each approach (bottom). This relative measure was constructed by subtracting the $P_{opt}(\widehat{D}^*)$ pertaining to the LASSO from that of the other methods within each combination of cancer type and $L_{\text{SUP}}$ value.

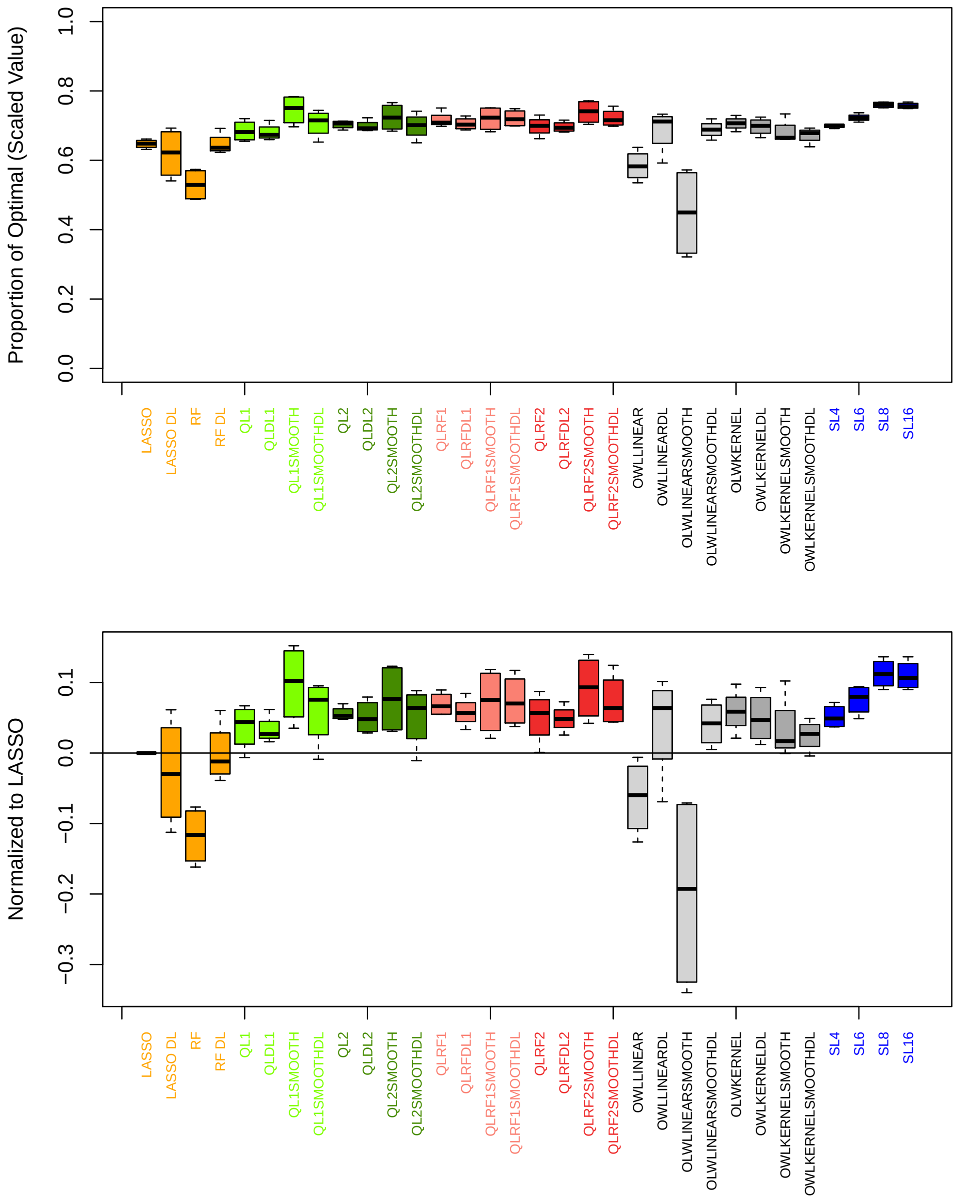


Figure 17: Overall performance with respect to each method and their variants in PDAC, pooled over cancer types and number of features utilized (top). $P_{opt}(\widehat{D}^*)$ for each method is normalized to the LASSO in each condition to highlight the relative performance of each approach (bottom). This relative measure was constructed by subtracting the $P_{opt}(\widehat{D}^*)$ pertaining to the LASSO from that of the other methods within each combination of cancer type and $L_{\mathrm{SUP}}$ value.

# 4 Results for Best Average Response and $P_{obs}(\widehat{D}^*)$

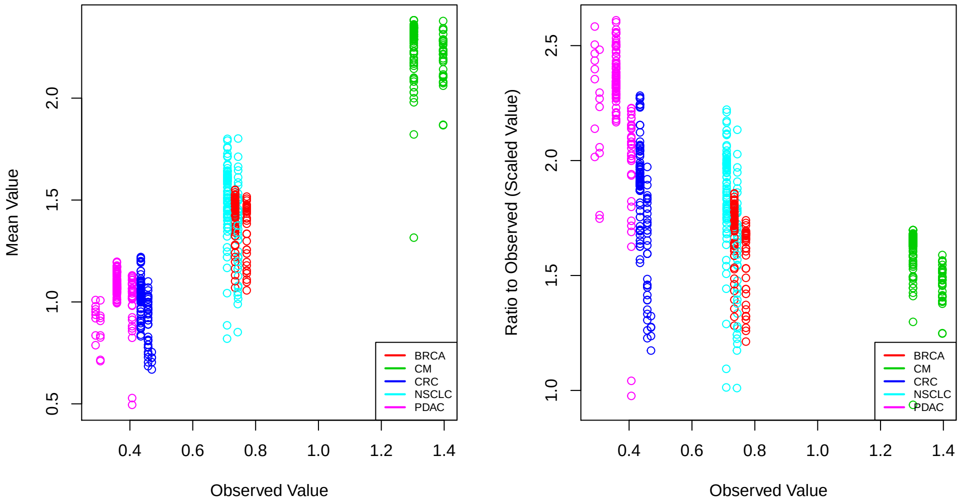


Figure 18: Original (left) and scaled (right) values corresponding to mean values from all analyses performed, encompassing each method, cancer type, and value of $L_{\text{SUP}}$ for Best Average Response. Observed values for each method (defined previously) vary significantly by cancer. The estimate of the optimal ITR in each method is correlated with the observed values across each cancer for each method. We normalize the mean values for each method by the observed values to allow for comparisons between cancers, defining this metric as "Ratio to Observed". This metric reflects how well a method performs in predicting treatment relative a randomly selected treatment.

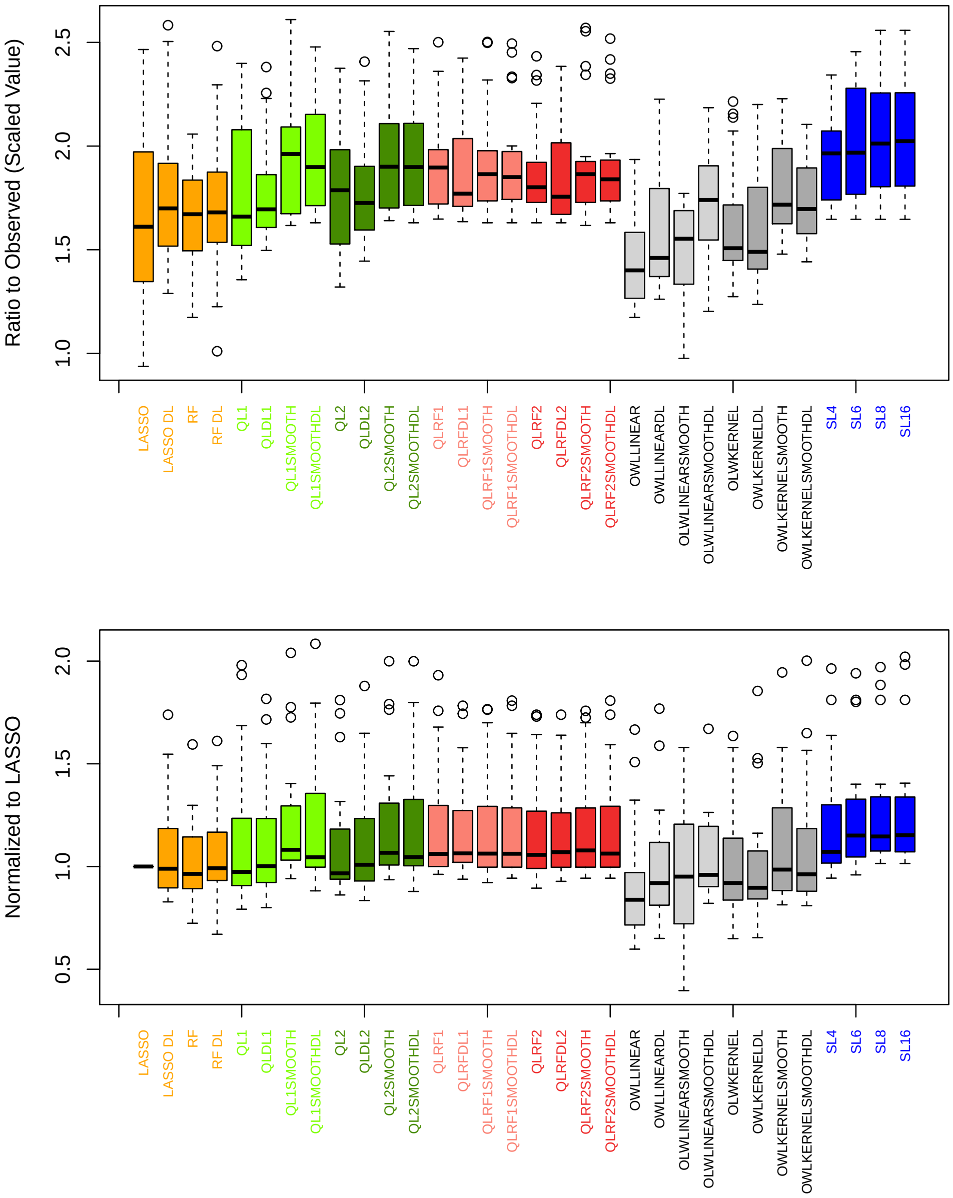


Figure 19: Overall performance with respect to each method and their variants, pooled over cancer types and number of features utilized (top). $P_{obs}(\widehat{D}^*)$ foor each method is normalized to the LASSO in each condition to highlight the relative performance of each approach (bottom). This relative measure was constructed by subtracting the $P_{obs}(\widehat{D}^*)$ pertaining to the LASSO from that of the other methods within each combination of cancer type and $L_{\text{SUP}}$ value.

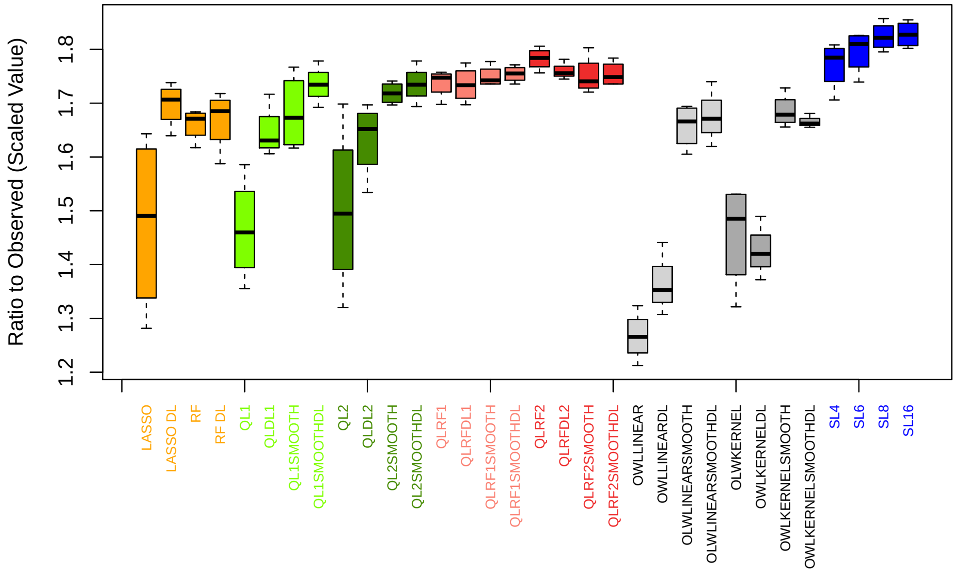


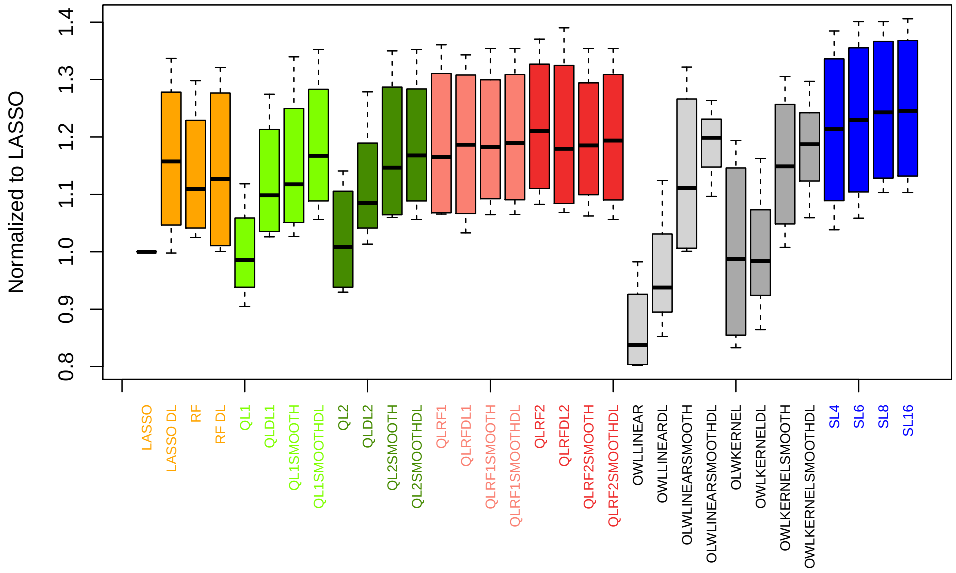


Figure 20: Overall performance with respect to each method and their variants in BRCA, pooled over cancer types and number of features utilized (top). $P_{obs}(\widehat{D}^{*})$ foor each method is normalized to the LASSO in each condition to highlight the relative performance of each approach (bottom). This relative measure was constructed by subtracting the $P_{obs}(\widehat{D}^{*})$ pertaining to the LASSO from that of the other methods within each combination of cancer type and $L_{\mathrm{SUP}}$ value.

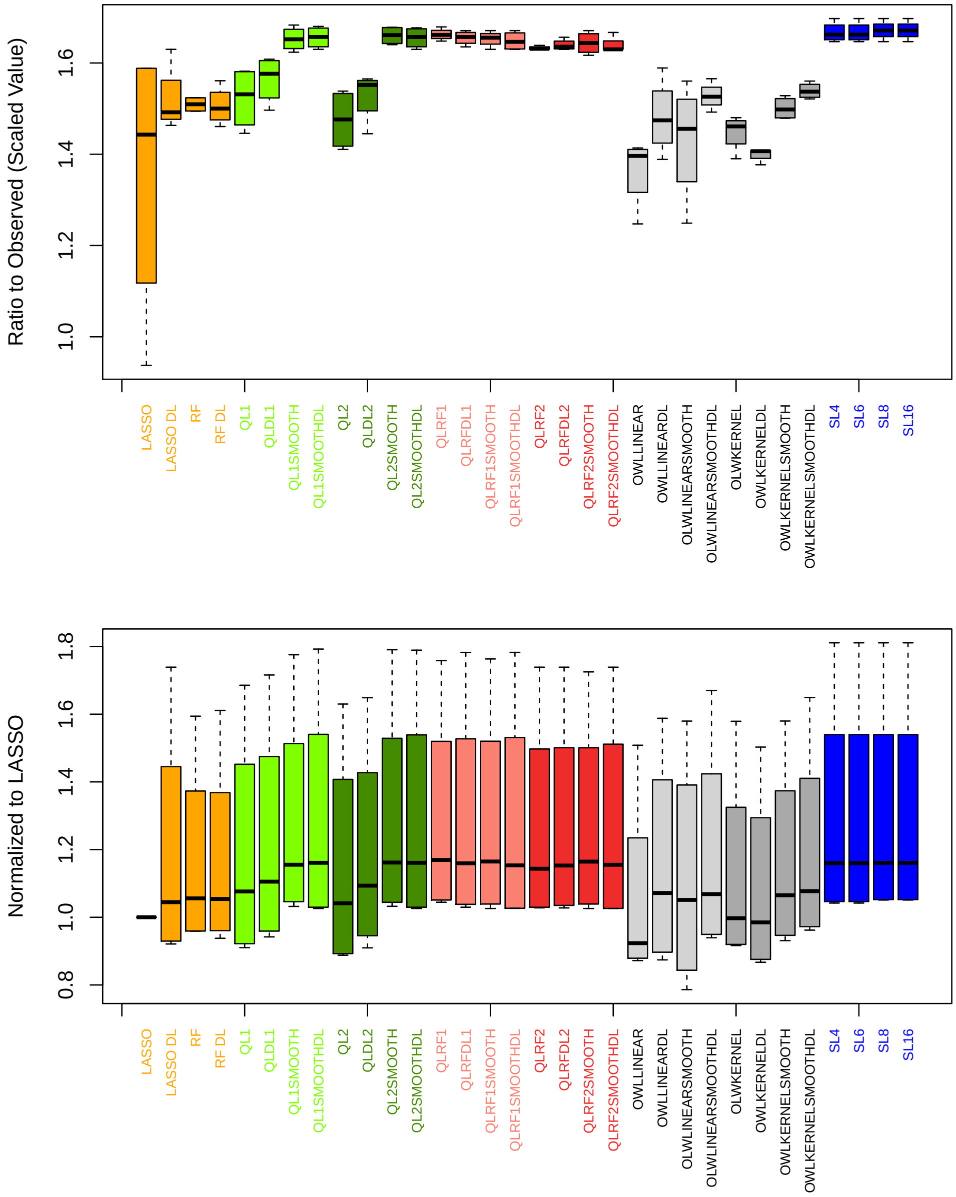


Figure 21: Overall performance with respect to each method and their variants in CM, pooled over cancer types and number of features utilized (top). $P_{obs}(\widehat{D}^{*})$ foor each method is normalized to the LASSO in each condition to highlight the relative performance of each approach (bottom). This relative measure was constructed by subtracting the $P_{obs}(\widehat{D}^{*})$ pertaining to the LASSO from that of the other methods within each combination of cancer type and $L_{\text{SUP}}$ value.

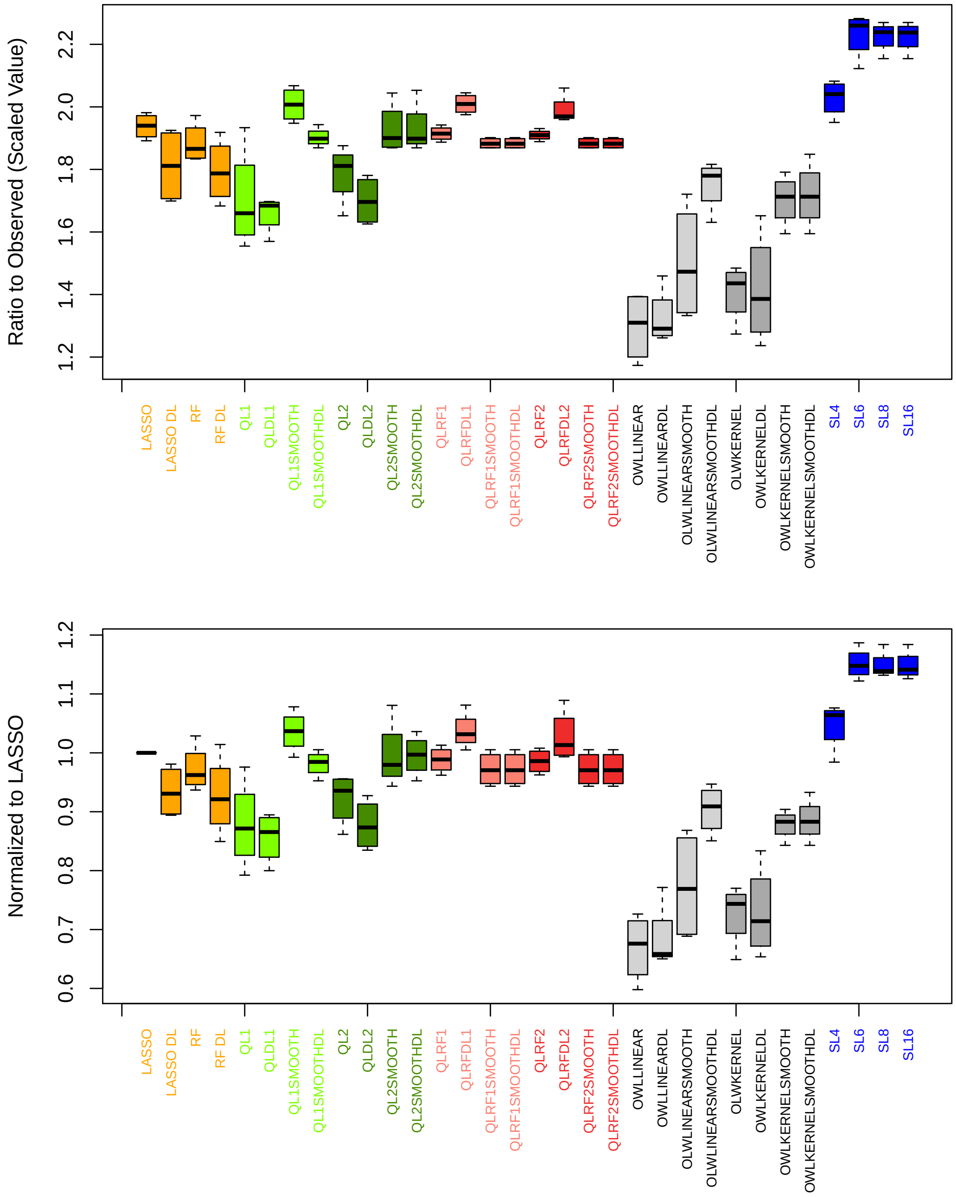


Figure 22: Overall performance with respect to each method and their variants in CRC, pooled over cancer types and number of features utilized (top). $P_{obs}(\widehat{D}^*)$ foor each method is normalized to the LASSO in each condition to highlight the relative performance of each approach (bottom). This relative measure was constructed by subtracting the $P_{obs}(\widehat{D}^*)$ pertaining to the LASSO from that of the other methods within each combination of cancer type and $L_{\text{SUP}}$ value.

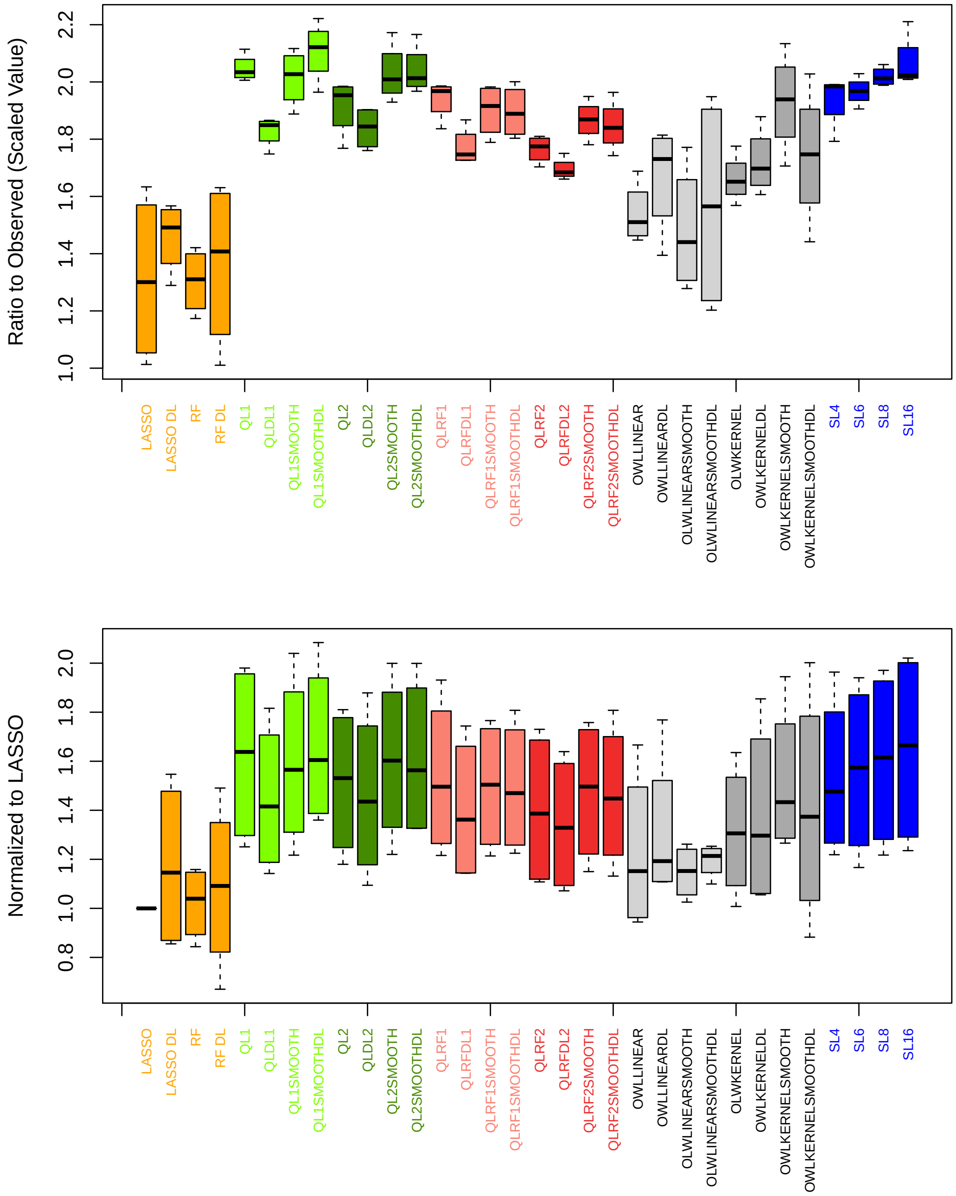


Figure 23: Overall performance with respect to each method and their variants in NSCLC, pooled over cancer types and number of features utilized (top). $P_{obs}(\widehat{D}^*)$ foor each method is normalized to the LASSO in each condition to highlight the relative performance of each approach (bottom). This relative measure was constructed by subtracting the $P_{obs}(\widehat{D}^*)$ pertaining to the LASSO from that of the other methods within each combination of cancer type and $L_{\mathrm{SUP}}$ value.

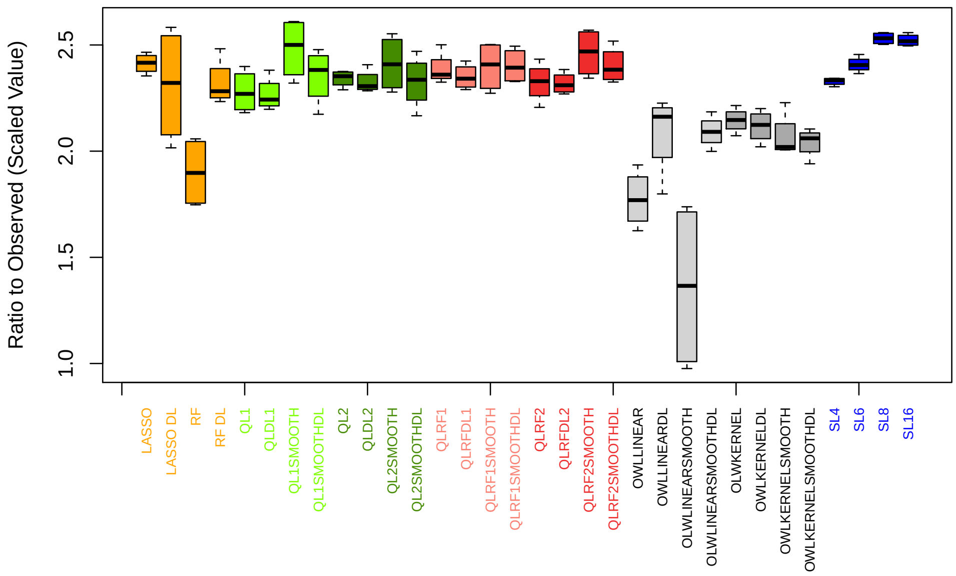


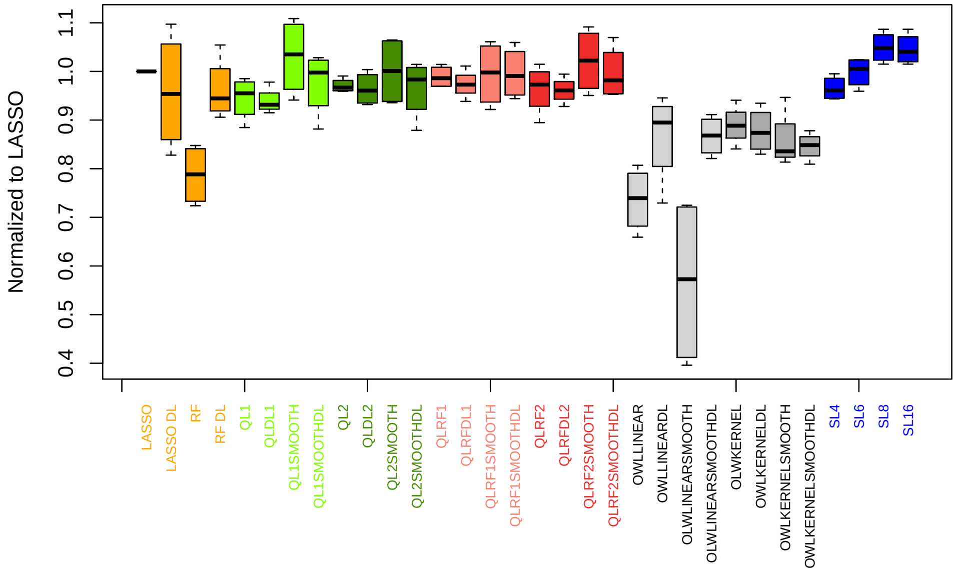


Figure 24: Overall performance with respect to each method and their variants in PDAC, pooled over cancer types and number of features utilized (top). $P_{obs}(\widehat{D}^*)$ foor each method is normalized to the LASSO in each condition to highlight the relative performance of each approach (bottom). This relative measure was constructed by subtracting the $P_{obs}(\widehat{D}^*)$ pertaining to the LASSO from that of the other methods within each combination of cancer type and $L_{\text{SUP}}$ value.

# 5 Results for Log Time to Doubling and $P_{opt}(\widehat{D}^*)$

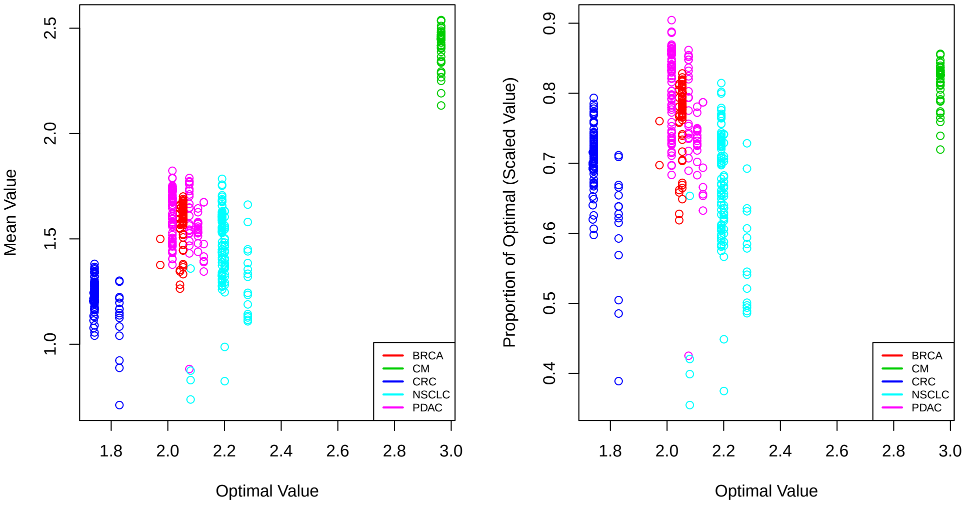


Figure 25: Original (left) and scaled (right) values corresponding to mean values from all analyses performed, encompassing each method, cancer type, and value of $L_{\text{SUP}}$ for log of TTD. Observed values for each method (defined previously) vary significantly by cancer. The estimate of the optimal ITR in each method is correlated with the observed values across each cancer for each method. We normalize the mean values for each method by the observed values to allow for comparisons between cancers, defining this metric as "Ratio to Observed". This metric reflects how well a method performs in predicting treatment relative a randomly selected treatment.

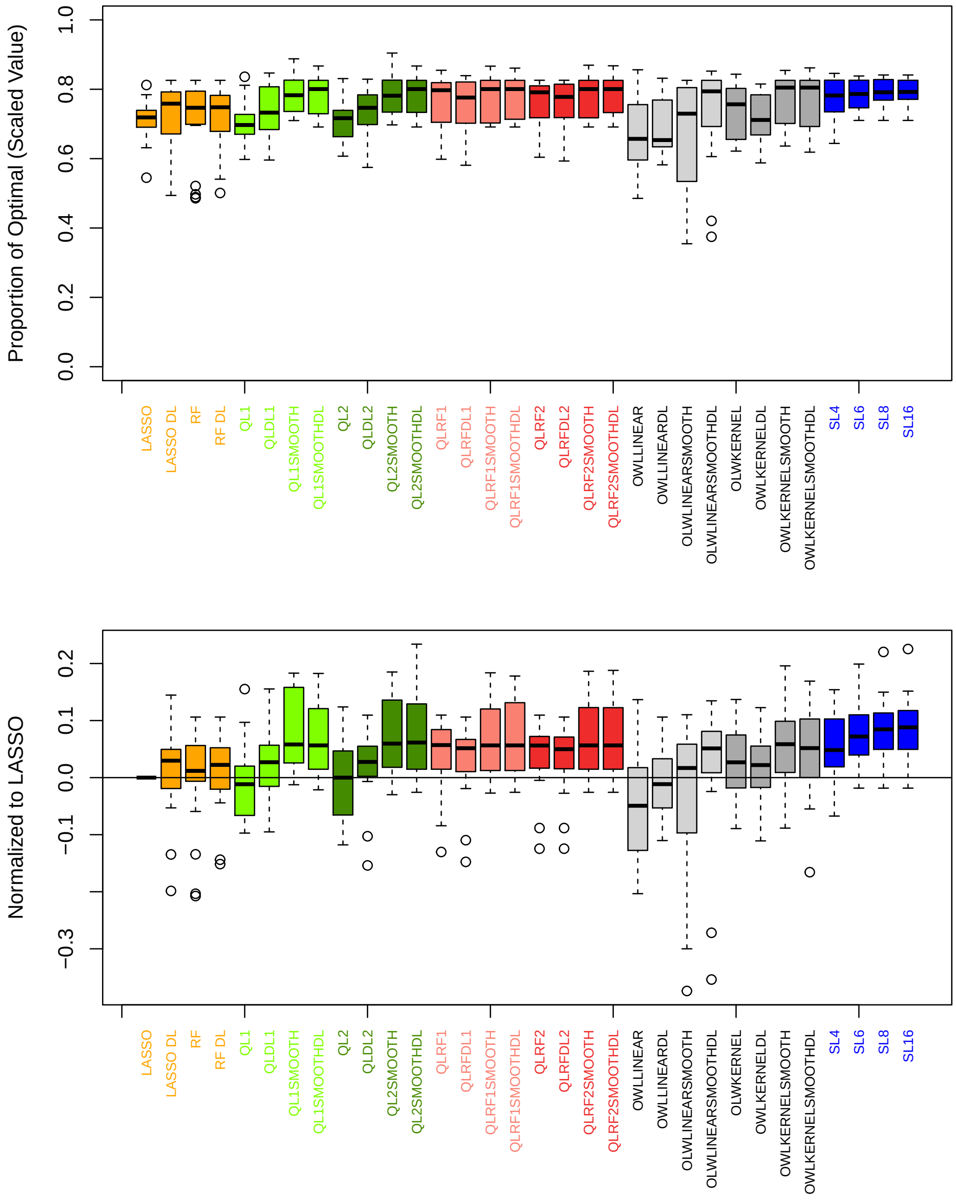


Figure 26: Overall performance (TTD) with respect to each method and their variants, pooled over cancer types and number of features utilized (top). $P_{opt}(\widehat{D}^*)$ foor each method is normalized to the LASSO in each condition to highlight the relative performance of each approach (bottom). This relative measure was constructed by subtracting the $P_{opt}(\widehat{D}^*)$ pertaining to the LASSO from that of the other methods within each combination of cancer type and $L_{\text{SUP}}$ value.

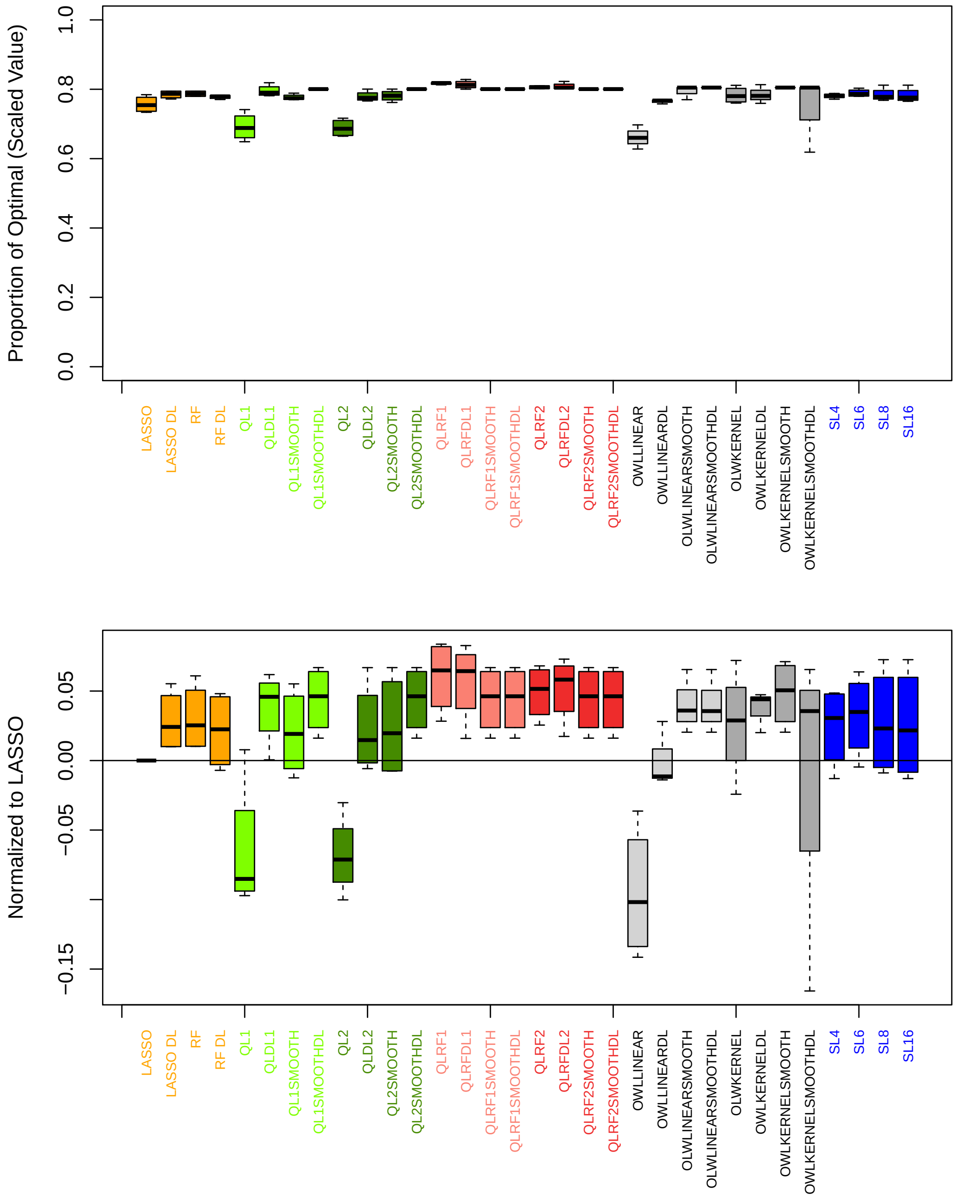

Figure 27: Overall performance (TTD) with respect to each method and their variants in BRCA, pooled over cancer types and number of features utilized (top). $P_{opt}(\widehat{D}^*)$ for each method is normalized to the LASSO in each condition to highlight the relative performance of each approach (bottom). This relative measure was constructed by subtracting the $P_{opt}(\widehat{D}^*)$ pertaining to the LASSO from that of the other methods within each combination of cancer type and $L_{\text{SUP}}$ value.

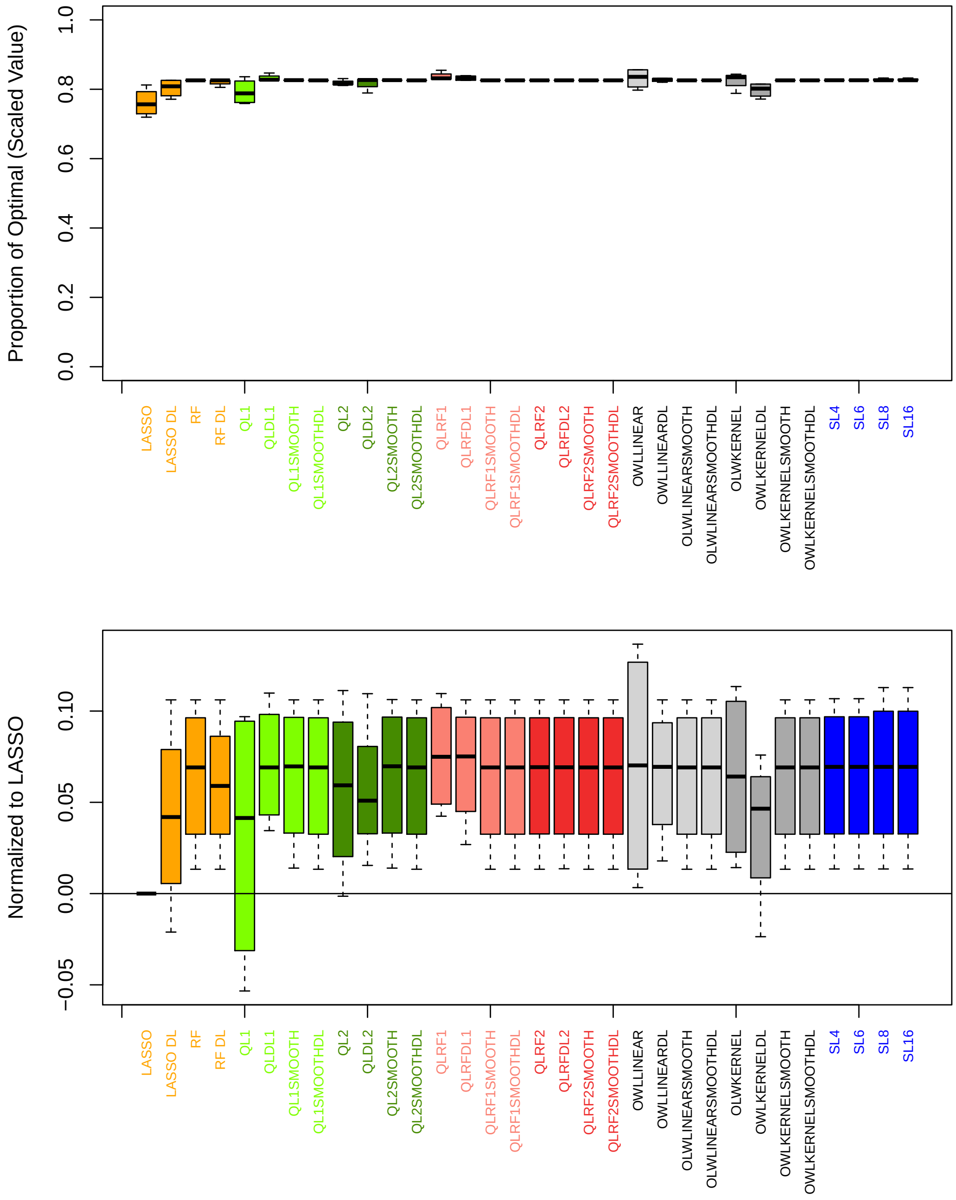


Figure 28: Overall performance (TTD) with respect to each method and their variants in CM, pooled over cancer types and number of features utilized (top). $P_{opt}(\widehat{D}^*)$ for each method is normalized to the LASSO in each condition to highlight the relative performance of each approach (bottom). This relative measure was constructed by subtracting the $P_{opt}(\widehat{D}^*)$ pertaining to the LASSO from that of the other methods within each combination of cancer type and $L_{\mathrm{SUP}}$ value.

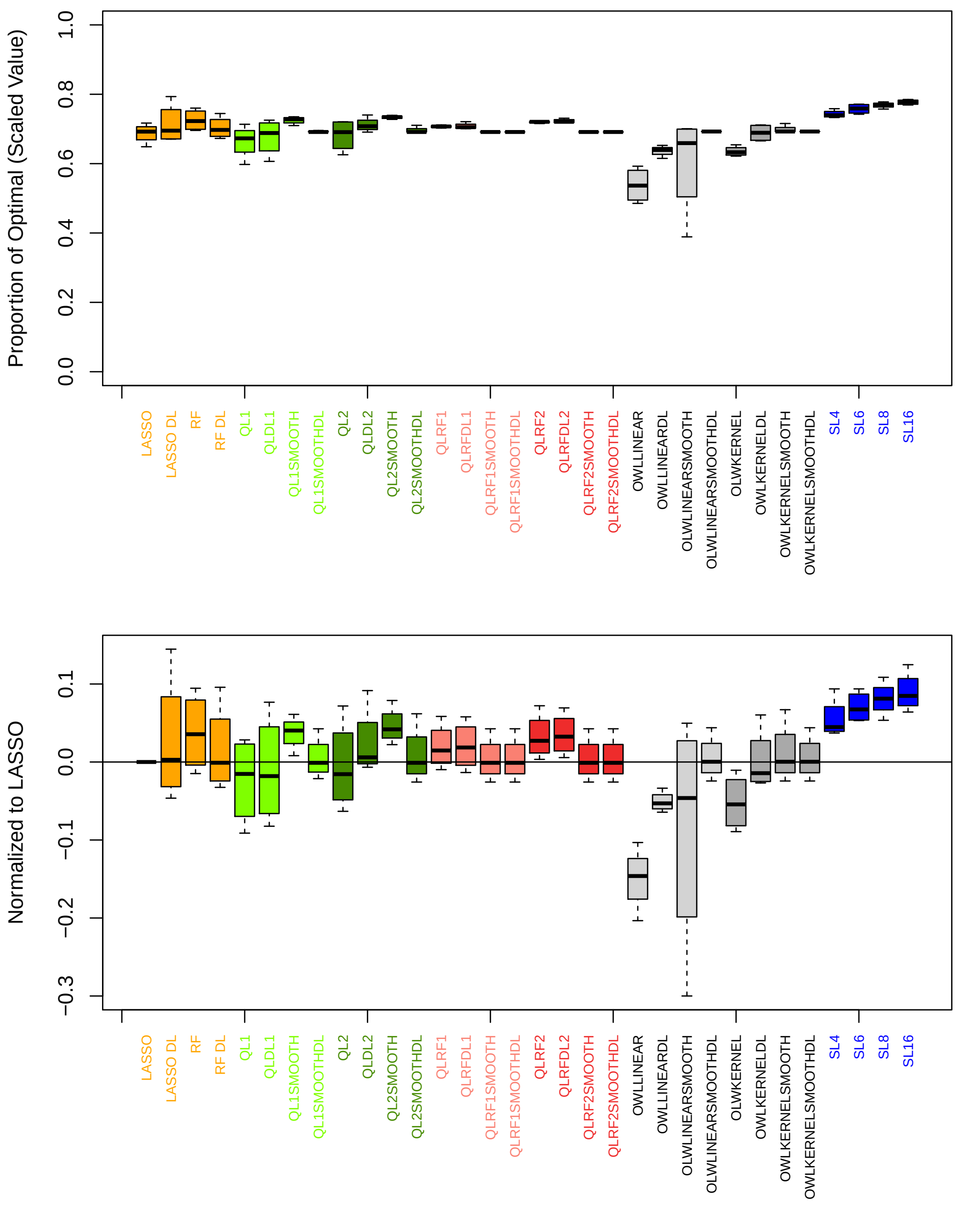


Figure 29: Overall performance (TTD) with respect to each method and their variants in CRC, pooled over cancer types and number of features utilized (top). $P_{opt}(\widehat{D}^*)$ for each method is normalized to the LASSO in each condition to highlight the relative performance of each approach (bottom). This relative measure was constructed by subtracting the $P_{opt}(\widehat{D}^*)$ pertaining to the LASSO from that of the other methods within each combination of cancer type and $L_{\text{SUP}}$ value.

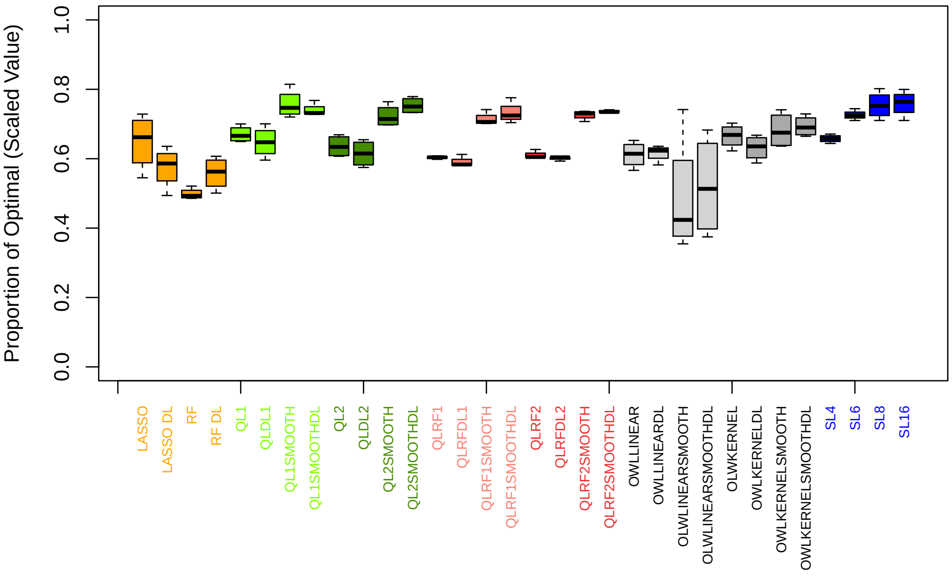


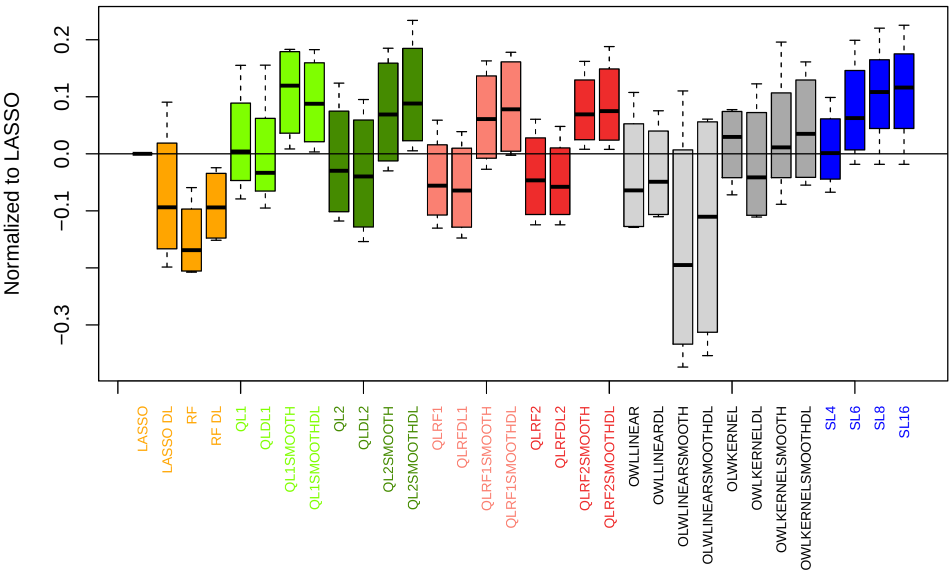


Figure 30: Overall performance (TTD) with respect to each method and their variants in NSCLC, pooled over cancer types and number of features utilized (top). $P_{opt}(\widehat{D}^*)$ for each method is normalized to the LASSO in each condition to highlight the relative performance of each approach (bottom). This relative measure was constructed by subtracting the $P_{opt}(\widehat{D}^*)$ pertaining to the LASSO from that of the other methods within each combination of cancer type and $L_{\text{SUP}}$ value.

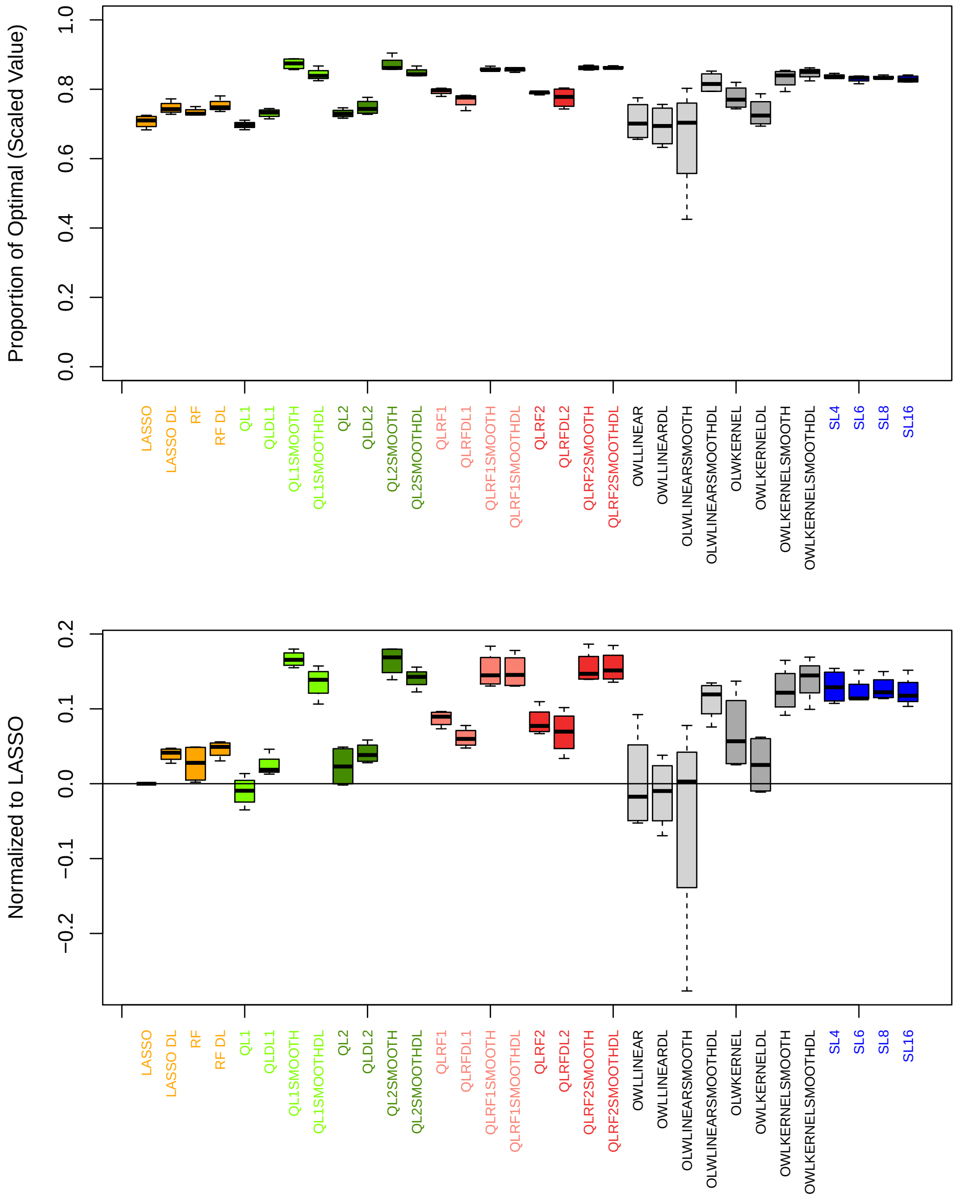


Figure 31: Overall performance (TTD) with respect to each method and their variants in PDAC, pooled over cancer types and number of features utilized (top). $P_{opt}(\widehat{D}^*)$ for each method is normalized to the LASSO in each condition to highlight the relative performance of each approach (bottom). This relative measure was constructed by subtracting the $P_{opt}(\widehat{D}^*)$ pertaining to the LASSO from that of the other methods within each combination of cancer type and $L_{\mathrm{SUP}}$ value.

# 6 Genomic platforms

## 6.1 RNA-seq

RNA-seq read counts are given only in FPKM format (Fragments per Kilobase per Million reads) for 399 PDX lines across 22665 genes, prior to filtering down to the 190 PDX lines with complete data. For a gene in a particular line, the number of sequenced reads pertaining to this gene is normalized by the total number of reads in that line (in millions) and the length of that particular gene (in kilobases). This allows for comparison of expressions between lines for a given gene (adjusted for sequencing depth bias), in addition to comparisons between genes in the same line (gene length bias, longer genes collect more sequenced reads at the same level of expression). FPKM values are log-transformed and then standardized within each gene prior to analysis. Upper Quartiles for the FPKM data look relatively stable and no strong evidence exists for aberrant lines (Supplementary Figure 32). Data is cleaned, no missing values or blank entries. More details can be found in Gao et al. (2015).

Figure 32: RNAseq FPKM summary per line

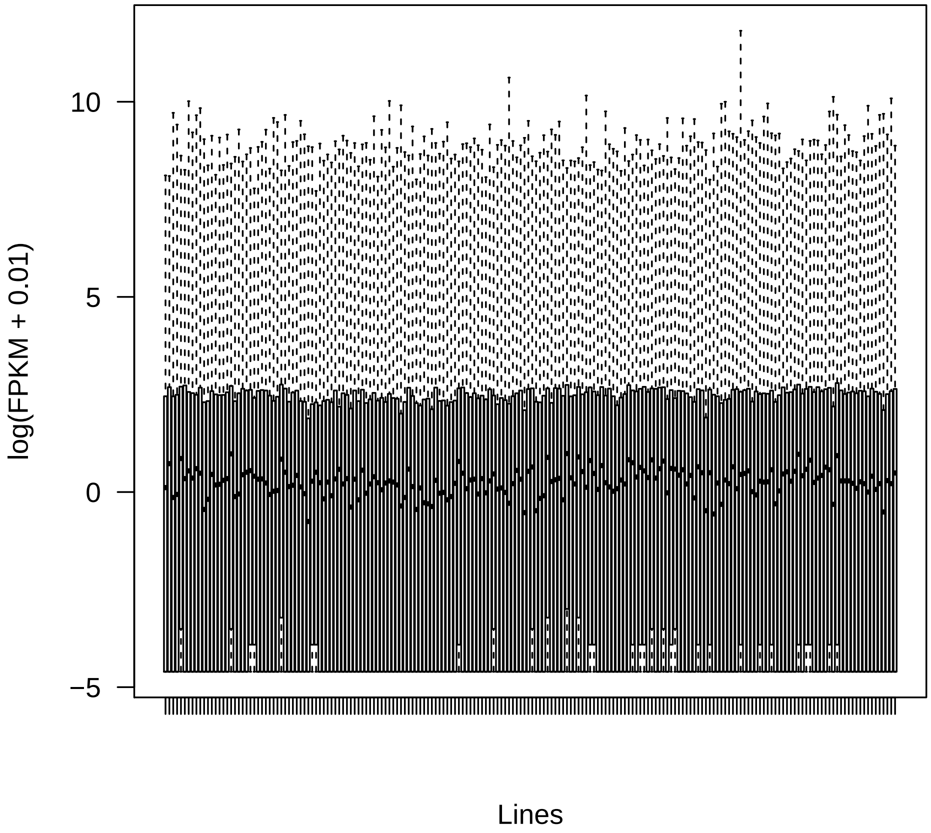

### 6.2 Copy Number data

Gene-level copy number estimates are provided for 375 lines across 23852 genes. Estimates are given in terms of the estimated number of copies of that particular gene. A value of 2 indicates normal copy number, less than 2 indicates a deletion event, and greater than 2 indicates an amplification of a gene's copy number. Both a copy-number segmentation file (not provided) and a gene-level copy-number value (provided) were generated using Partek Genomic Suite 6.6 genomic segmentation algorithm (Partek, Inc.). CIN scores (first two rows of data matrix) were calculated as the s.d. of the mean copy-number across chromosome arms. Boxplots of gene copy number scores for each line demonstrate significant variability in copy number across individuals (Supplementary Figure 33.)

Figure 33: Copy Number summary per line

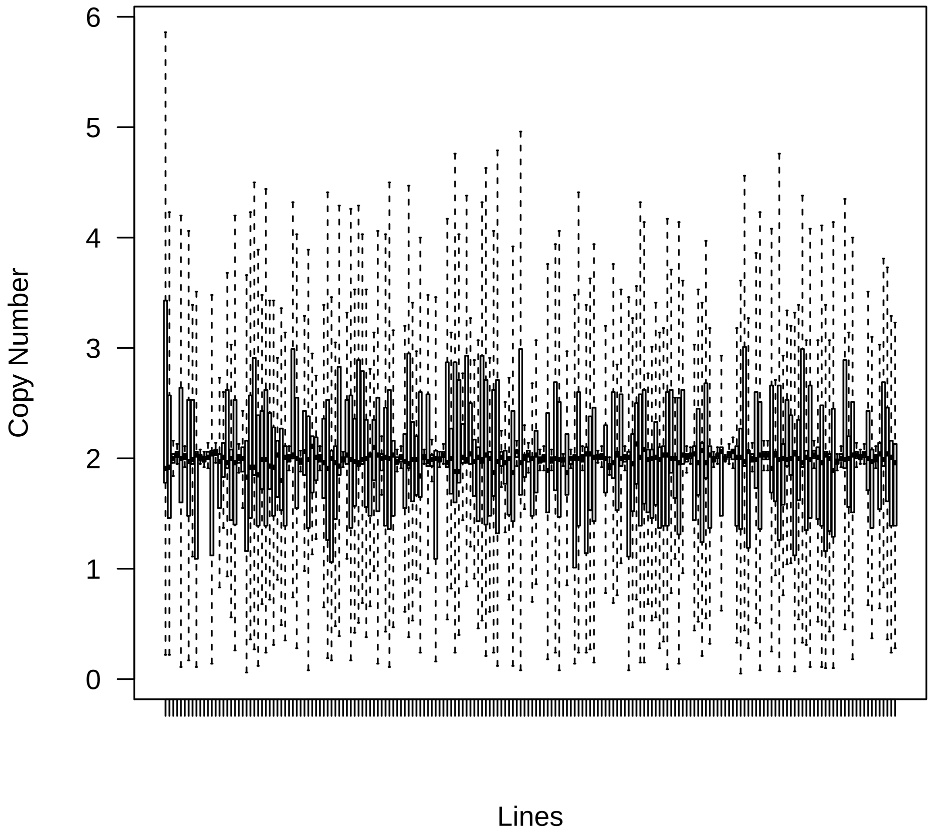

### 6.3 Mutation data

Mutation and filtered copy number data is provided for 399 lines. The Category column in the provided file lists whether the entry is either Amp5 (copy number amplification between 5 and 8), Amp8 (copy number amplification greater than 8), Del0.8 (copy number deletion less than 0.8), MutKnownFunctional (known function mutation), MutLikelyFunctional (likely functional mutation), and MutNovel (novel mutations). Relative frequencies of each across PDX lines with complete data is give in Supplementary Figure 34. We find that the median number of individual mutations found per line is approximately 200 mutations, and that the median number of times a gene is found to be mutated across lines (having at least one mutation in that gene) is 3 times out of 190 lines. For specific individual mutations in genes, this value drops to 1, however there are a small subset of mutations that commonly mutated across lines that may be utilized (mutations in genes such as TP53, MAP3K4, MUC4, APC, KRAS). Going forward for each gene we create a binary indicator taking value of 1 if at least one mutation is found in that gene and line, and 0 otherwise.

## 7 Supplementary Methods

### 7.1 Unsupervised Screening

Unsupervised screening on the set of available genomic features is performed to remove features with low variability, low expression, or low frequency, as these features will likely not be helpful for prediction. Available genomic features include RNA-seq gene expression measurements in log FPKM (Fragments Per Kilobase per Million Reads), gene copy number estimates, and a binary variable indicating the presence/absence of any mutations occurring in gene $l$, $l = 1, \ldots, L_{TOT}$. We define $L_{TOT}$ as the number of genes with features available from at least one of the three data types. Gene expression features are removed if they have on average $< 1$ FPKM across all PDX lines pertaining to a particular cancer $k$, as these low-expressing genes may not be reliable in their expression or have a strong biological impact (Love et al., 2014). We rank the remaining gene expression features based upon their variability across PDX lines within a cancer (median absolute deviation) and remove those features in the bottom quintile, as these low variance features may be less informative for prediction (Hackstadt and Hess, 2009). We perform a similar filtering to remove

Figure 34: Mutation and filtered CN summary per line

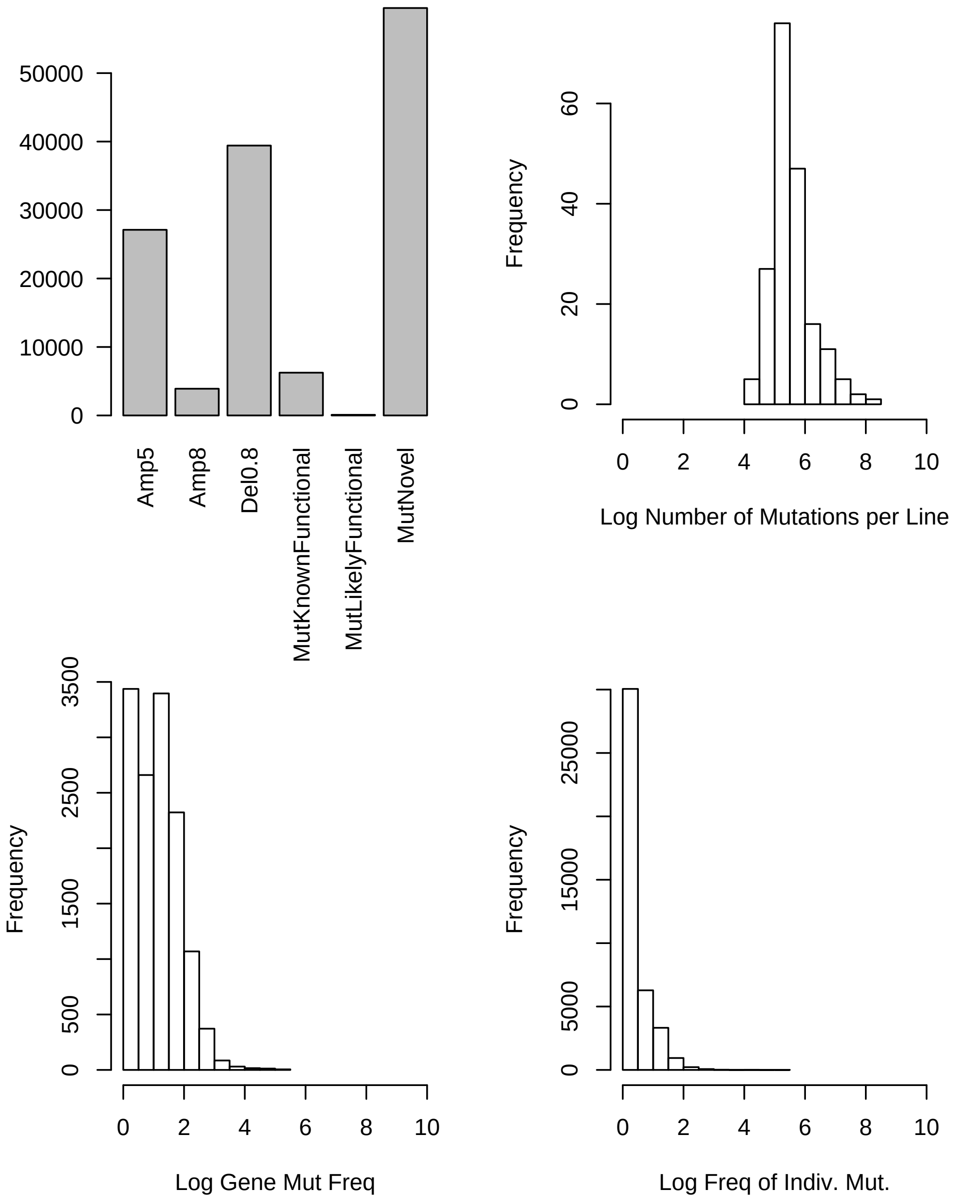

low variance features from the copy number dataset. Lastly, we remove mutations present in less than 10% or greater than 90% of PDX lines in a particular cancer. The number of features prior to and following unsupervised screening is detailed in the Supplementary Table 2, where we define $L_{\text{UNSUP}}$ as the number of genes in cancer $k$ with at least one feature remaining from the set of gene expression, copy number, and mutation features available from the study.

Unsupervised screening on treatments is also performed to remove treatments not consistently applied across PDX lines (within cancers). Treatments that were utilized in less than 90% of PDX lines within a cancer type are removed, as these treatments were likely discontinued due to excessive toxicity or dosing issues.

After this screening, we denote the observed vector of remaining predictors corresponding to gene $l$ for PDX line $j$ and cancer $k$ as $X_{jk,l}$, $l = 1, \ldots, L_{\text{UNSUP}}$. Here $X_{jk,l}$ may have dimension $p = 1, 2, 3$, depending on the number of genomic features for gene $l$ that remain after unsupervised screening. We also define $\tilde{Y}_{ijk}$ as the $q = 2$ dimensional vector of outcomes for the $ijk^{th}$ mouse, where $\tilde{Y}_{ijk} = (Y_{ijk,1}, Y_{ijk,2})$, $Y_{ijk,1}$ is the observed Best Average Response for mouse $ijk$, and $Y_{ijk,2}$ is the observed log Time to Tumor Doubling for mouse $ijk$. Recall that each mouse $i$ in cancer $k$ was given the same treatment across lines $j = 1, \ldots, m_k$. Note that each PDX line has a unique set of predictors that are shared among the $i = 1, \ldots, P_k$ mice from that line, as they originated from the same patient tumor.

## 7.2 Supervised Screening Based on Pairwise Treatment-Gene Interactions

After unsupervised screening, we further screen the genomic features pertaining to each of the remaining $L_{\text{UNSUP}}$ genes in order to jointly assess their prognostic and predictive effects. Gene-level screening was performed separately for each cancer and treatment, whereby the union of all remaining predictors across treatments and cancers were retained. We used two supervised screening methods to assess prognostic and predictive effects: Brownian Distance Correlation (BDC) and Canonical Correlation (CCA).

To perform screening based on the prognostic effects, we consider each treatment and each gene $(i, l)$ within cancer $k$, then calculate the BDC and CCA between $X_{jk,l}$ and $\tilde{Y}_{ijk}$ across all PDX lines $(j = 1, ..., m_k)$. The BDC is $\mathcal{V}_n^2(i, l) = \|\phi^n_{X_{jk,l},\tilde{Y}_{ijk}}(t, s) - \phi^n_{X_{jk,l}}(t)\phi^n_{\tilde{Y}_{ijk}}(s)\|^2$, where $n = m_k$, for any random variable $X$,

$\phi_X^n = \mathbb{E}_n\left[e^{it'X}\right]$ with $\mathbb{E}_n$ denoting the empirical measure from $n = m_k$ PDX lines, and $\|\cdot\|$ is a suitable norm. When $X_{jk,l}$ and $\tilde{Y}_{ijk}$ are independent,

$$n\mathcal{V}_n^2 \xrightarrow[n\to\infty]{D} \|\zeta(t,s)\|^2, \tag{1}$$

where $\zeta(\cdot,\cdot)$ is a complex-valued Gaussian random process with mean 0 and a known covariance function (Székely et al., 2009). Therefore, using (1), we can obtain $p$-values for a test of independence between $X_{jk,l}$ and $\tilde{Y}_{ijk}$.

For CCA (Hotelling, 1936), we first compute the canonical correlations between $X_{jk,l}$ and $\tilde{Y}_{ijk}$ based on the empirical estimates for the covariance matrices and cross-covariance between $X_{jk,l}$ and $\tilde{Y}_{ijk}$, denoted as $\hat{\rho}_1, \hat{\rho}_2, ..., \hat{\rho}_J$ where $J$ is the minimum of the dimensions of $X_{jk,l}$ and $\tilde{Y}_{ijk}$, so that $\hat{\rho}_1$ is the largest correlation between two linear combinations of $X_{jk,l}$ and $\tilde{Y}_{ijk}$, and $\hat{\rho}_2$ is the largest correlation of the linear combinations which are uncorrelated with the ones yielding a correlation of $\hat{\rho}_1$ and so on. To test whether $X$ and $Y$ are correlated, we employ the test statistic

$$H_n = -\left\{n - 1 - \frac{1}{2}(p+q+1)\right\}\log\left\{\prod_{j=1}^{J}(1-\hat{\rho}_j^2)\right\}.$$

We empirically compute a p-value based on this test via permutation testing, similar to Székely et al. (2009).

We also use BDC and CCA to assess the predictive power of each genomic feature variable, in terms of whether the difference of the outcomes from two different treatments is related to the genomic feature. For each possible pair of treatments, say $i$ and $i'$, $i' = 1, \ldots, P_k$ and $i \neq i'$, we test whether there is any association between $X_{jk,l}$ and $\tilde{Y}_{ijk} - \tilde{Y}_{i'jk}$ using BDC and CCA.

After conducting the above tests, each gene $l$ is left with $P_k$ prognostic and $P_k(P_k - 1)/2$ predictive p-values. We rank genes on the basis of their minimum BDC p-value, using the magnitude of the corresponding CCA value in the case of ties. To assess the impact of the size of the predictor space used for ITR estimation, we use our ranking system to create datasets of the top $L_{\text{SUP}}$ candidate genes and their associated genomic features, where $L_{\text{SUP}} = 50, 100, 500,$ and $1000$ genes from both the prognostic and predictive screenings. We detail the number of features remaining for each $L_{\text{SUP}}$ value in Supplementary Table 2.

## 7.3 Dimension Reduction via Deep Learning

For a particular cancer $k$, we obtain $p_{L_{\text{SUP}}}$ features pertaining to the $L_{SUP}$ top ranked genes following unsupervised and supervised screening steps, where $L_{SUP} = 50, 100, 500, 1000$ (Supplementary Table 2). Here we consider one further step of dimension reduction for each of the datasets produced by supervised screening: Deep Autoencoders (DAE), a variant of deep neural networks (Vincent et al., 2010). This method builds a complex nonlinear prediction model to predict all the feature variables using only a low-dimensional representation of all the feature variables. In this way, the resulting model takes advantage of intrinsic relationships between the features to rely more heavily on those features that successfully predict the remainder. In our application of DAE to a set of $p_{L_{\text{SUP}}}$ predictors in a cancer $k$, we reduce the dimension listed in Supplementary Table 2 to those listed in Supplementary Table 5.

Specifically, let $X$ denote all genomic feature variables from the supervised screening step. Then $X \in \mathbb{R}^{p_{L_{SUP}}}$, where $p_{L_{SUP}}$ is the total number of genomic features pertaining to the $L_{SUP}$ genes that remain after the supervised screening. A DAE takes $X$ as both input and output and adopts a neural network with multiple hidden layers to predict $X$ using $X$. In this analysis, we use a DAE with three hidden layers and index the layers of the DAE by $s = 0, \ldots, 4$, where $s = 0$ corresponds to the input layer $X$, $s = 1, 2, 3$ correspond to the hidden layers, and $s = 4$ corresponds to the output layer. Let layer $s$ of the DAE, $H_s$, contain $n_s$ nodes, such that $H_s = (h_1^s, \ldots, h_{n_s}^s)$, $s = 1, \ldots, 4$. Then the DAE model takes the form

$$h_u^s = \tanh\left(H_{s-1}' w_u^s + b_u^s\right), \tag{2}$$

where $u = 1, \ldots, n_s$ indexes the nodes of layer $s$, $s = 1, \ldots, 4$, $w_u^s$ is an $n_{s-1} \times 1$ vector of weights relating $h_u^s$ to $H_{s-1}$ such that $w_u^s = (w_{1u}^s, \ldots, w_{n_{s-1},u}^s)$, and $b_u^s$ is the $s$th element of the bias vector at layer $s$. To estimate all the weights, DAE minimizes a group LASSO penalized square loss between the predicted value from this neural network and the output $X$, and this minimization is carried out via a stochastic gradient decent algorithm incorporating both forward and back propagation. In particular, during the back

propagation, both $w$'s and $b$'s are updated according to

$$\begin{cases} w_u^s \leftarrow w_u^s - \eta \frac{\partial C}{\partial w_u^s} \\ b_v^s \leftarrow b_v^s - \eta \frac{\partial C}{\partial b_v^s} \end{cases}, \tag{3}$$

where $C$ is the objective function and $\eta$ is the step size of gradient descent called the learning rate (LeCun et al., 2015). As a note, the group LASSO penalty term in $C$ induces the sparsity of $w_u^s$ at the level of individual features of $H_0$ (Wang and Laber, 2017).

For our application, we fix the numbers of neurons for the first and third hidden layers as $n_1 = n_3 = p_{L_{SUP}}/2$ and let the output dimension $n_4 = p_{L_{\text{SUP}}}$. The size of the second hidden layer, $n_2$, is chosen by cross-validation, as is the initial value of the learning rate $\eta$. We train each DAE for 27000 epochs, or full passes through the data. Each of these epochs comprises $\lceil p_{L_{SUP}}/15 \rceil$ steps of stochastic gradient descent with a batch size of 15. In each step, the gradients in (3) are estimated using batches of 15 randomly chosen observations, rather than the entire data, to enhance computational speed. The learning rate $\eta$ is decayed to 90% of its current value after every 5000 steps to help prevent overfitting. After model training, we extract the second hidden layer of the DAE as the reduced-dimension dataset, resulting in a new $n_2$-dimensional predictor matrix.

## 7.4 Adaptations of Off the Shelf Methods for ITR estimation

An alternative approach is to directly obtain the prediction models for the outcomes using all treatments and genomic feature variables, without using the estimated tree structure for the treatments. In particular, we apply random forests and a linear model with LASSO penalty to achieve this aim, and compare the performance of these methods to those from the previous section.

We construct the predictor matrix and response for the Random Forest model as follows. For each centered treatment response vector $R_{ik}$, we define $\mathbf{X}_{ik}$ as the $m_k \times p_{L_{\text{SUP}}}$ matrix of genomic features. We note that this matrix is identical for $i = 1, \ldots, P_k$ since the mice pertaining to the same PDX line share the same set of genomic data. We then append an $(m_k) \times P_k$ matrix of indicator variables $\mathbf{T}_{ik}$ to $\mathbf{X}_{ik}$ to give us $\mathbf{X}_{aug,ik} = (\mathbf{X}_{ik}, \mathbf{T}_{ik})$, where the $i$th column of $\mathbf{T}_{ik} = 1$ and is 0 otherwise, indicating that treatment $a_i$ was

applied to $R_{ik}$. We obtain the final $(m_k P_k) \times P_k$ response vector $R_k$ such that $R_k = (R'_{1k}, \ldots, R'_{P_k k})'$ and our final predictor matrix $\mathbf{X}_{aug,k} = (\mathbf{X}'_{aug,1k}, \ldots, \mathbf{X}'_{aug,P_k k})'$, stacking the treatment vectors and predictor matrices for treatments $i = 1, \ldots, P_k$. Given $R_k$ and $\mathbf{X}_{aug,k}$, we fit a random forests model to obtain $\widehat{E}_{RF}(R^*(a)|\mathbf{X}_{aug,k})$. Then, the estimated optimal decision rule assigns the treatment predicted to yield the greatest reward, such that

$$\widehat{D}^{RF}(x) = \underset{a \in \{a_1, \ldots, a_{P_k}\}}{\arg\max} \widehat{E}_{RF}(R^*(a)|x),$$

where x is the covariate vector consisting of genomic predictors and treatment indicator vector corresponding to $a$. That is, the treatment which maximizes the expected clinical outcome $\widehat{E}_{RF}(R^*(a)|x)$ given the fitted model and genomic features in a new patient is selected as the optimal treatment under $\widehat{D}^{RF}(x)$.

Similarly, we fit a linear model with LASSO penalty to the PDX data. In this case, the matrix of predictors includes the first-order interactions between treatments and genomic features, where $\mathbf{X}_{aug,ik} = (\mathbf{X}_{ik}, \mathbf{T}_{ik}, \mathbf{XT}_{ik})$ and $R_k$ and $\mathbf{X}_{aug,k}$ is constructed as described previously. Here $\mathbf{XT}_{ik}$ represents the matrix containing the pairwise interactions between $\mathbf{X}_{ik}$ and $\mathbf{T}_{ik}$. The specific value of the LASSO tuning parameter is chosen via cross-validation (see Main Text Section 3.4). The estimated ITR is

$$\widehat{D}^{LASSO}(x) = \underset{a \in \{a_1, \ldots, a_{p_k}\}}{\arg\max} \widehat{E}_{LASSO}(R^*(a)|x),$$

where again the treatment which maximizes the expected clinical outcome given the fitted model is selected as the optimal treatment.

# References


Gao, H., Korn, J. M., Ferretti, S., Monahan, J. E., Wang, Y., Singh, M., Zhang, C., Schnell, C., Yang, G., Zhang, Y. et al. (2015), "High-throughput Screening Using Patient-derived Tumor Xenografts to Predict Clinical Trial Drug Response," *Nature Medicine*, 21(11), 1318–1325.

Hackstadt, A. J., and Hess, A. M. (2009), "Filtering for Increased Power for Microarray Data Analysis,"

*BMC Bioinformatics*, 10(1), 11.

Hotelling, H. (1936), "Relations Between Two Sets of Variates," *Biometrika*, 28(3/4), 321–377.

LeCun, Y., Bengio, Y., and Hinton, G. (2015), "Deep Learning," *Nature*, 521(7553), 436–444.

Love, M. I., Huber, W., and Anders, S. (2014), "Moderated Estimation of Fold Change and Dispersion for RNA-seq Data with DESeq2," *Genome Biology*, 15(12), 550.

Székely, G. J., Rizzo, M. L. et al. (2009), "Brownian Distance Covariance," *The Annals of Applied Statistics*, 3(4), 1236–1265.

Vincent, P., Larochelle, H., Lajoie, I., Bengio, Y., and Manzagol, P.-A. (2010), "Stacked Denoising Autoencoders: Learning Useful Representations in a Deep Network with a Local Denoising Criterion," *Journal of Machine Learning Research*, 11(Dec), 3371–3408.

Wang, L., and Laber, E. (2017), "Sufficient Markov Decision Processes," *Submitted*, .
